# Supplementary material for: Specula: Scaling formal specifications for autonomous model checking of system code
Source: arXiv:2607.25333 source file (2026-08-03)
Supplement: Supplementary file 1 [file 02_bug_report.tex]

\section{Example \specula Bug Report}
\label{app:bug-report}

The following is an example of the bug reports \specula creates: this covers the second bug presented in Section \ref{sec:libgomp-case-study}.
It includes the bug scenario and motivation, root causes and a conjecture at why this bug was missed by developers, code references, a reproduction, a model checking and trace validation summary, and a suggested fix to facilitate manual review.

\begin{promptboxwithheader}{libgomp Bug Report}
    \begin{Verbatim}[breaklines=true, breakanywhere=true]
# Missing BAR_TASK_PENDING in omp_fulfill_event (Deadlock)

`omp_fulfill_event` from an unshackled thread wakes a barrier thread without setting BAR_TASK_PENDING, which can lead to a deadlock.

Affects all GCC versions since 11 (commit d656bfda, Feb 2021) and all barrier implementations (centralized, flat, POSIX) -- they all use identical BAR_TASK_PENDING gating.

## Root Cause

In `libgomp/task.c`, the `omp_fulfill_event` function has two wake paths:

**Path 1 -- dependent tasks exist (`new_tasks > 0`)**: Correctly sets BAR_TASK_PENDING before waking (fixed in [commit ba886d0c](https://github.com/gcc-mirror/gcc/commit/ba886d0c488ebea2eb2df95c2069a3e207704dac), May 2021):
```c
if (new_tasks > 0)
  {
    gomp_team_barrier_set_task_pending (&team->barrier);  // <- correct
    do_wake = team->nthreads - team->task_running_count;
  }
```

**Path 2 -- no dependent tasks, unshackled thread (`!shackled_thread_p`)**: Only wakes, does NOT set BAR_TASK_PENDING (introduced in [commit d656bfda](https://github.com/gcc-mirror/gcc/commit/d656bfda2d8316627d0bbb18b10954e6aaf3c88c), Feb 2021):
```c
if (!shackled_thread_p
    && !do_wake
    && team->task_detach_count == 0
    && gomp_team_barrier_waiting_for_tasks (&team->barrier))
  do_wake = 1;  // missing gomp_team_barrier_set_task_pending
```

## Why This Causes Deadlock

The barrier wait loop (same pattern in all 3 barrier implementations) uses BAR_TASK_PENDING as the gate for entering `gomp_barrier_handle_tasks`:

```c
// config/linux/bar.c (centralized barrier, lines 113-125):
do {
    do_wait ((int *) &bar->generation, generation);
    gen = __atomic_load_n (&bar->generation, MEMMODEL_ACQUIRE);
    if (__builtin_expect (gen & BAR_TASK_PENDING, 0))  // <- gate
        gomp_barrier_handle_tasks (state);
    generation |= gen & BAR_WAITING_FOR_TASK;
} while (!gomp_barrier_state_is_incremented (gen, state));
```

`gomp_barrier_handle_tasks` is not only responsible for running tasks -- it also calls `gomp_team_barrier_done` when `task_count == 0`, which appears to be the main path for completing a barrier when tasks are involved.

The deadlock sequence:
1. Detached task body completes -> task becomes `GOMP_TASK_DETACHED`, `task_count > 0`
2. All team threads enter barrier wait loop, see no tasks to run, enter `futex_wait`
3. External thread calls `omp_fulfill_event` -> `task_count` drops to 0
4. `gomp_team_barrier_wake` wakes one thread via `futex_wake`
5. BAR_TASK_PENDING is not set, so `bar->generation` remains unchanged
6. Woken thread loads `bar->generation`, sees no change, loops back to `futex_wait`
7. **DEADLOCK** -- no thread ever calls `gomp_team_barrier_done`

Key insight: `futex_wake` only wakes threads from `futex_wait`; it does **not** change `bar->generation`. Without BAR_TASK_PENDING modifying `bar->generation`, the wake is a no-op from the woken thread's perspective.

## Reproduction

**File**: `repro/detach_fulfill_deadlock.c`

The reproduction uses only standard OpenMP 5.0 `detach` clause and POSIX `pthread_create`. Its structure is similar to GCC's own test case `task-detach-13.c` ([commit ba886d0c](https://github.com/gcc-mirror/gcc/commit/ba886d0c488ebea2eb2df95c2069a3e207704dac)), but without `depend` clauses (to exercise the `new_tasks == 0` path).

```bash
gcc -fopenmp -O2 -lpthread -o detach_repro detach_fulfill_deadlock.c

# Deadlocks with any GCC (system or NVIDIA-patched):
timeout 5 ./detach_repro
echo $?  # 124 = deadlock

# Succeeds with patched libgomp:
timeout 5 LD_LIBRARY_PATH=/path/to/patched/.libs ./detach_repro
echo $?  # 0 = success
```

**Tested**: 5/5 deadlock (unpatched) vs 5/5 success (patched), using identical source/compiler/flags builds differing only by the one-line fix.

## Suggested Fix

Add `gomp_team_barrier_set_task_pending` before `do_wake = 1` in the unshackled thread path:

```c
if (!shackled_thread_p
    && !do_wake
    && team->task_detach_count == 0
    && gomp_team_barrier_waiting_for_tasks (&team->barrier))
  {
    gomp_team_barrier_set_task_pending (&team->barrier);
    do_wake = 1;
  }
```

This is the same pattern used in:
- The `new_tasks > 0` path (task.c, same function, 3 lines above)
- `gomp_target_task_completion` (task.c:835)

### Patch

See `repro/patches/bug29-fulfill-event-set-task-pending.patch`

## TLA+ Model

The bug was discovered through TLA+ model checking. The specification extends the flat barrier model with detached task lifecycle:
- `ScheduleDetachTask`: models `#pragma omp task detach(ev)` -- task enters the queue
- `DetachTaskBodyComplete`: task body finishes, task becomes `GOMP_TASK_DETACHED` (`taskDetachCount++`, `taskPending` cleared)
- `FulfillEvent`: external thread calls `omp_fulfill_event` -- `taskCount--`, `taskDetachCount--`, but **`taskPending` stays unchanged** (the bug)
- `WaitingPrimaryCompleteBarrier`: primary re-enters `gomp_barrier_handle_tasks` from wait loop when `taskPending` is set

Key invariant violated: `DetachFulfillNoDeadlock` -- asserts that the system never reaches a state where all threads are in the barrier wait loop (`pc[t] = "waiting"`), `taskCount = 0`, `waitingForTask = TRUE`, and `~taskPending`. This state is a deadlock because no thread will enter `gomp_barrier_handle_tasks` to call `gomp_team_barrier_done`.

The counterexample trace (13 states) shows the exact deadlock sequence:
1. Detach task scheduled -> `taskCount=1`, `taskPending=TRUE`
2. All threads enter barrier, primary scans, all arrived
3. Primary enters `handle_tasks` (`waitingForTask=TRUE`)
4. Task body completes -> `taskDetachCount=1`, `taskPending=FALSE` (queue empty)
5. Primary sees no runnable tasks, exits to wait loop (`pc[Primary]="waiting"`)
6. `FulfillEvent`: `taskCount->0`, but `taskPending` stays `FALSE`
7. **Deadlock**: all threads waiting, `taskCount=0`, `~taskPending` -- invariant violated

Applying the fix (`taskPending' = TRUE` in `FulfillEvent`) eliminates the violation: TLC explores 662 states with no errors.

## Discussion

This is an understandably easy issue to miss:

1. **Narrow test coverage gap**: The existing test `task-detach-13.c` uses `depend(out/in)`, which triggers the `new_tasks > 0` path (correctly fixed by ba886d0c). The `new_tasks == 0` + unshackled thread combination is a less common scenario that hasn't been covered yet.
2. **Subtle `futex_wake` semantics**: It's natural to expect that `futex_wake` + `do_wake = 1` would be sufficient to unblock a waiting thread. The subtlety is that `futex_wake` doesn't modify `bar->generation`, so without BAR_TASK_PENDING the woken thread sees no change and loops back to sleep.
3. **Incremental development**: The `set_task_pending` pattern (ba886d0c, May 2021) was added 3 months after the original unshackled-thread code (d656bfda, Feb 2021), but only to the `new_tasks > 0` path. The symmetric `!shackled_thread_p` path could benefit from the same treatment.

## Reproduction Instructions

See `repro/README.md` for step-by-step reproduction instructions.
    \end{Verbatim}
\end{promptboxwithheader}
