# Supplementary material for: Specula: Scaling formal specifications for autonomous model checking of system code
Source: arXiv:2607.25333 source file (2026-08-03)
Supplement: Supplementary file 2 [file 03_false_positives.tex]

\section{RQ1: False Positives}
\label{app:rq1-fp}

This section includes descriptions of the two false positives: one in dotnet/dotNext, and one in databendlabs/openraft.
Both of these false positives reported a potential issue that could follow should a certain exceptional behaviour occur; this exception itself was prevented by other codepaths.
These false positives were reported by a development version of \specula that did not include automated bug confirmation.
This motivated us to develop Phase 4 and include developer intent analysis.

\subsection{dotnet/dotNext Raft Bug}

The following is an excerpt from the bug report.

\begin{quote}
    \emph{
The three async void state transition methods (MoveToFollowerState, MoveToCandidateState, MoveToLeaderState) call MoveToStandbyState() in their catch blocks as a fallback. If MoveToStandbyState() itself throws (e.g., DisposeAsync failure during UpdateStateAsync), the exception escapes the async void method and crashes the process via the unobserved exception handler.
    }
\end{quote}

The following is the maintainer's response.

\begin{quote}
    \emph{
\textsf{DisposeAsync} as well as \textsf{Dispose} must be idempotent and exception-free. This is recommended not only for Raft, it is for all implementations of \textsf{IDisposable} and \textsf{IAsyncDisposable} interfaces. In .NEXT Raft, every Raft state is designed in that way. It's better to analyze their implementations to achieve the necessary behavior rather than assuming the exception.
    }
\end{quote}

\subsection{databendlabs/openraft Bug}

The following is an excerpt from the bug report.
\begin{quote}
    \emph{
\textsf{update\_vote()} in \textsf{establish\_leader()} is only checked with \textsf{debug\_assert!()}, which gets compiled out in release builds. If \textsf{update\_vote} fails (e.g., due to a higher-term uncommitted vote from a rejected response arriving between quorum grant and leader establishment), \textsf{state.vote} silently diverges from \textsf{leader.vote}. The practical impact is limited (leader core paths use \textsf{self.leader}), but it causes \textsf{is\_leader()} to return false and metrics to be inaccurate.
    }
\end{quote}

The following are excerpts of the maintainer's response.
\begin{quote}
    {\em
        [\dots] I believe the \textsf{update\_vote} call in \textsf{establish\_leader()} cannot actually fail in a valid execution — that's precisely why it's guarded by \textsf{debug\_assert} rather than explicit error handling.

        Here's why: whenever \textsf{state.vote} is updated to a higher vote from a different node, \textsf{update\_internal\_server\_state()} calls \textsf{become\_following()}, which clears both \textsf{self.leader} and \textsf{self.candidate}. Once the candidate is cleared, any subsequent vote response is simply ignored (\textsf{handle\_vote\_resp} returns early), so \textsf{establish\_leader()} is never reached.

        The \textsf{debug\_assert} is intentional: if it ever fires, it signals a consensus invariant violation, and the program should be terminated immediately rather than continuing in a potentially inconsistent state. [\dots]

        Looking at your test, it fabricates an impossible scenario by injecting Vote(T7, 0, committed) into node 1 via a fake AppendEntries heartbeat. [\dots] 
        }
\end{quote}
