# Supplementary material for: Specula: Scaling formal specifications for autonomous model checking of system code
Source: arXiv:2607.25333 source file (2026-08-03)
Supplement: Supplementary file 3 [file 06_libgomp.tex]

\section{RQ1: libgomp Case Study Confirmation}
\label{app:libgomp-case-study}
The following is an anonymized excerpt from an email to the GCC mailing list from an NVIDIA engineer.

\begin{quote}
    {\em
Also -- I wanted to mention that the team working on \specula very kindly 
looked at these patches to search for any problems.
(\specula is an AI powered framework using TLA+ to find bugs in system 
    code [\dots]).

    They found a bug in `\textsf{gomp\_team\_barrier\_wait\_for\_tasks}` where I had 
    missed that the `\textsf{BAR\_CANCELLED}` flag could have been set on a ``final'' 
barrier -- when it gets cleared by the primary thread adjusting the 
generation (to say that all threads should be held) the assertion at 
line 521 triggers.

The observable behaviour outside of the assertion failure would have 
been that a secondary thread ``waiting'' on the primary thread would have 
been unnecessarily spinning and taking up CPU resources.

Since the fix is a simple change of the loop to remove the 
    `\textsf{BAR\_CANCELLED}` flag from the local `generation` number I plan to 
include the fix in the respin I assume I'll have to make once these 
patches have had review, but I figured it worth highlighting to any 
reviewer nonetheless.

The testcase \specula generated also triggers the assertion at line 384, 
since that loop has the same assumption.

-----
N.b. they have also found another bug that seems legitimite in the 
existing OpenMP codebase.  They raised it here: [\dots]
    }
\end{quote}
