# Supplementary material for: Specula: Scaling formal specifications for autonomous model checking of system code
Source: arXiv:2607.25333 source file (2026-08-03)
Supplement: Supplementary file 4 [file 07_bug_descriptions.tex]

\section{RQ3: Full Bug Descriptions}
\label{app:rq3-bugs-full}

Table \ref{tab:rq3-bugs-full} contains expanded descriptions of the bugs identified during RQ3 ablations, as well as which \specula configs successfully identified the bug.
All bugs had already been previously identified by \specula runs prior to the controlled experiments, except the view advance bug in Autobahn.

\begin{table}[H]
\centering
\caption{Descriptions of bugs reported in ablations.}
\label{tab:rq3-bugs-full}
\resizebox{\columnwidth}{!}{%
\begin{tabular}{llll}
\hline
\textbf{Project} & \textbf{Bug}                                 & \textbf{ID'ed by}                                                     \\ \hline
autobahn & QC does not bind to proposal value & \begin{tabular}[c]{@{}l@{}}\specula,\\ no-bug-families,\\ no-phase-1\end{tabular}      \\ \hline
autobahn         & TC verification always returns Ok            & \begin{tabular}[c]{@{}l@{}}\specula,\\ no-bug-families\end{tabular}  \\ \hline
autobahn         & No duplicate guard for Confirm votes         & \begin{tabular}[c]{@{}l@{}}\specula,\\ no-bug-families\end{tabular}  \\ \hline
autobahn         & View advance side-effect on rejected Prepare & \specula                                                             \\ \hline
autobahn         & Agreement violation (composition)            & \specula                                                             \\ \hline
autobahn         & Winning view selection bug                   & no-phase-1                                                           \\ \hline
libgomp          & gomp\_sem\_wait race                         & \specula                                                             \\ \hline
libgomp          & Priority inversion                           & \specula                                                             \\ \hline
libgomp          & BAR\_CANCELLED lost on no-task fast path     & \specula                                                             \\ \hline
papaya           & Wrong parker deadlock on resize abort        & \begin{tabular}[c]{@{}l@{}}\specula,\\ no-bug-families\end{tabular}  \\ \hline
\end{tabular}%
}
\end{table}
