# Supplementary material for: Specula: Scaling formal specifications for autonomous model checking of system code
Source: arXiv:2607.25333 source file (2026-08-03)
Supplement: Supplementary file 5 [file 09_prompts.tex]

\section{\specula Prompts}
\label{app:prompts}

\specula's agentic design relies heavily on prompts.
Sections \ref{app:prompts-phase1} through \ref{app:prompts-phase4} contain the main prompts for each of the phases, along with the Agent Skill prompts.

\onecolumn

\subsection{Phase 1: Repository Mining}
\label{app:prompts-phase1}
\begin{promptboxwithheader}{Phase 1 Launch Prompt}
    \begin{Verbatim}[breaklines=true, breakanywhere=true]
# Code Analysis Task

You are analyzing the following system:

- **Name**: ${name}
- **GitHub**: ${github_short}
- **Language**: ${language}
- **Reference Algorithm**: ${reference}
- **Repository**: ${repo_dir}
- **Working Directory**: ${work_dir}

## Instructions

Follow the **code-analysis** skill methodology. Read the skill guide at:
  ${SPECULA_ROOT}/.claude/skills/code_analysis/guide.md

Then read the reference files as needed:
  ${SPECULA_ROOT}/.claude/skills/code_analysis/references/bug-archaeology.md
  ${SPECULA_ROOT}/.claude/skills/code_analysis/references/deep-analysis.md
  ${SPECULA_ROOT}/.claude/skills/code_analysis/references/distributed-analysis.md
  ${SPECULA_ROOT}/.claude/skills/code_analysis/references/concurrent-analysis.md
  ${SPECULA_ROOT}/.claude/skills/code_analysis/references/modeling-brief-format.md

And see the example:
  ${SPECULA_ROOT}/.claude/skills/code_analysis/examples/hashicorp-raft-modeling-brief.md

## Phases

Execute all 4 phases in order:

1. **Reconnaissance** -- Build structural map of codebase and classify the target as Category A (distributed/message-passing) or Category B (concurrent/lock-free/runtime)
2. **Bug Archaeology** -- Mine git history and GitHub issues/PRs for bugs
3. **Deep Analysis** -- Systematic code reading to find new issues
4. **Modeling Brief** -- Synthesize findings into modeling-brief.md

## Output

Write your outputs to:
- `${work_dir}/modeling-brief.md` -- The primary deliverable (handoff to Spec Generation)
- `${work_dir}/analysis-report.md` -- Detailed audit trail of all findings

## Critical Rules

1. VERIFY before reporting. Re-read code. Check for compensating mechanisms. No unverified claims.
2. Read issue DISCUSSIONS, not just titles. For any issue you plan to reference, read the full comment thread via \`gh issue view --comments\` to confirm it hasn't been debunked.
3. Do NOT hallucinate code logic. If unsure, READ IT. Cite file:line for every claim.
4. Use parallel Task subagents aggressively. Launch multiple subagents concurrently for: issue batch verification (5-10 issues per subagent), file-by-file deep analysis (one subagent per core file), and commit review. This is essential for both depth AND coverage.
5. Evidence-based claims only. Show code, git commits, issue discussions, or code path inconsistencies.
6. Bug Families over flat lists. Group by mechanism. 5 actionable families > 17 flat findings.
7. Every finding must be classified: model-checkable, test-verifiable, or code-review-only.
8. Thoroughness is non-negotiable. Analyze ALL bug-fix commits touching core files. Deeply read 30+ GitHub issues (full discussion threads). Report coverage statistics in the analysis report.
9. Record the system category and justification in \`modeling-brief.md\`. Later phases should not have to rediscover whether this is Category A or B.
10. After classification, follow the matching category-specific reference file under \`skills/code_analysis/references/\`. Do not force a distributed-system template onto a concurrent library, or vice versa.
    \end{Verbatim}
\end{promptboxwithheader}

\begin{promptboxwithheader}{Phase 1 Agent Skill Prompt}
    \begin{Verbatim}[breaklines=true, breakanywhere=true]
# Code Analysis for Formal Verification

Investigate a system implementation to find bugs. Some bugs can be confirmed directly (copy-paste errors, data races). The most critical bugs -- protocol safety violations -- need TLA+ model checking to verify. The **Modeling Brief** captures findings and plans how to verify them.

## Input / Output

**Input**: Repository path + reference algorithm/paper (optional) + GitHub URL (optional)

**Output**: `modeling-brief.md` (handoff to Spec Generation) + `analysis-report.md` (optional audit trail)

**The user drives each phase.** You provide methodology and execute on their direction.

---

## Step 0: Classify System Category

Before archaeology or deep analysis, classify the target as one of:

- **Category A (Distributed / Message-Passing)** -- network RPC, disk I/O, cluster membership, protocol state machines
- **Category B (Concurrent / Lock-Free / Runtime)** -- CAS loops, atomics, thread handoff, memory reclamation, ownership transfer, async cancellation

Record the category and a brief justification in `modeling-brief.md`.

After classifying:

- read `references/deep-analysis.md` for the shared methodology
- read `references/distributed-analysis.md` for **Category A**
- read `references/concurrent-analysis.md` for **Category B**

---

## Phase 1: Reconnaissance

**Goal**: Build a structural map -- core modules, scale, concurrency model, and atomicity boundaries.

---

## Phase 2: Bug Archaeology

**Goal**: Map historical bugs to identify error-prone areas and recurring patterns. This phase requires **thorough** coverage -- the quality of the entire analysis depends on the evidence gathered here.

### Steps

1. **Git history mining** by keyword (fix, bug, race, panic, deadlock, correctness, crash, corrupt, leak, inconsistent, wrong). Analyze **all** significant bug-fix commits, not just a sample.
2. **Issue/PR verification** -- read full discussions, not just titles. Use `gh issue list` with multiple keyword searches and label filters to maximize coverage.
3. **Bug Family grouping** -- group by shared **mechanism**, not by file.
4. **Reference comparison** (if applicable) -- find deviations from paper/other implementations.

### Depth Requirements

- **Git commits**: Analyze all bug-fix commits touching core files. Report the total count.
- **GitHub issues**: Read the full discussion thread (including all comments) for every issue you plan to reference. Aim to deeply read **30+ issues** for a medium-sized project. Report: total issues collected, total deeply read, total confirmed, total excluded as false positive.
- **Open PRs**: Review all open PRs with bug-fix intent -- they often contain fixes waiting for review and reveal known-but-unfixed problems.
- **Parallelization**: Use **multiple Task subagents in parallel** for issue verification (batch 5-10 issues per subagent). Do NOT read issues sequentially -- this wastes time.

**Read `references/bug-archaeology.md`** for detailed methodology.

---

## Phase 3: Deep Analysis

**Goal**: Find new issues through systematic code reading, guided by Phase 2 -- code path inconsistencies, non-atomic operations, missing guards, reference deviations.

### Parallelization Strategy

Deep Analysis is the most time-consuming phase. **Use parallel Task subagents aggressively**:

- Launch one subagent per major source file (e.g., state machine, replicator, persistence, snapshot)
- Each subagent reads its file completely and applies all analysis patterns
- After all subagents return, cross-reference findings in the main context

For a codebase with 6+ core files, aim for **4-6 parallel subagents** in the deep analysis phase.

### Verification

Every finding MUST be verified: re-read exact code lines, check for compensating mechanisms, trace execution path, check if it's an acknowledged design decision.

**Read `references/deep-analysis.md`** for the full methodology.

---

## Phase 4: Modeling Brief

**Goal**: Synthesize findings into an actionable document for Spec Generation -- select top Bug Families, propose spec extensions, state what NOT to model and why, classify remaining findings by verification method.

**Read `references/modeling-brief-format.md`** for the format specification.
**See `examples/hashicorp-raft-modeling-brief.md`** for a complete example.

---

## Critical Rules

1. **VERIFY before reporting.** Re-read the code. Check for compensating mechanisms. No unverified suspicions.
2. **Read issue discussions, not just titles.** For every issue you reference, read the full comment thread via `gh issue view --comments`. Confirm it hasn't been debunked.
3. **Do NOT hallucinate code logic.** If unsure, READ IT. Cite `file:line` for every claim.
4. **Exclude false positives explicitly.** Explain WHY each exclusion was made.
5. **Use parallel subagents aggressively.** Launch multiple Task subagents for concurrent issue verification, concurrent file analysis, and concurrent commit review. This is essential for both depth AND coverage.
6. **Evidence-based claims only.** Show code, git commits, issue discussions, or code path inconsistencies.
7. **Bug Families over flat lists.** Group by mechanism. 5 actionable families > 17 flat findings.
8. **Thoroughness is non-negotiable.** Do not skip issues, truncate commit analysis, or sample instead of scanning. The analysis report should document coverage statistics (total commits analyzed, issues deeply read, false positives excluded).
9. **Classify Category A vs B explicitly.** Carry that decision into the Modeling Brief. Later phases should not have to rediscover it.

---

## Reference Files

- **`references/bug-archaeology.md`** -- Git mining and issue verification methodology
- **`references/deep-analysis.md`** -- Shared deep-analysis methodology
- **`references/distributed-analysis.md`** -- Category A (distributed / message-passing) analysis patterns
- **`references/concurrent-analysis.md`** -- Category B (concurrent / lock-free / runtime) analysis patterns
- **`references/modeling-brief-format.md`** -- Standard format for the handoff document
- **`examples/hashicorp-raft-modeling-brief.md`** -- Complete real-world example

## Related Skills

- **spec-generation** -- Next phase: produces TLA+ specs from the Modeling Brief
- **tla-trace-workflow** -- Validates the trace spec against real traces

## Additional References

For additional examples beyond the built-in ones, see the [Specula case-studies repository](https://github.com/specula-org/specula-case-studies) which contains 60+ completed case studies across distributed systems, consensus protocols, and concurrent data structures.
    \end{Verbatim}
\end{promptboxwithheader}

\subsection{Phase 2: Initial Spec Generation}
\label{app:prompts-phase2}
\begin{promptboxwithheader}{Phase 2 Launch Prompt}
    \begin{Verbatim}[breaklines=true, breakanywhere=true]
# TLA+ Spec Generation Task

You are generating a TLA+ specification for: **${name}**

## Inputs

- **Modeling Brief**: ${brief}
- **Source Code**: ${repo_dir}
- **Output Directory**: ${spec_dir}

## Instructions

Follow the **spec-generation** skill methodology. Read the skill guide at:
  ${SKILL_DIR}/guide.md

Then read the reference files:
  ${SKILL_DIR}/references/base-spec-methodology.md
  ${SKILL_DIR}/references/mc-spec-pattern.md
  ${SKILL_DIR}/references/trace-spec-pattern.md
  ${SKILL_DIR}/references/instrumentation-spec-format.md

Before writing specs, read `${brief}` and determine whether this target is Category A (distributed/message-passing) or Category B (concurrent/lock-free/runtime). If it is Category B, shape the spec around thread-local state, linearization points, stale views, memory ordering, reclamation, and ownership transfer. Do not force a message-bag / protocol-state template onto the code.

## Phases

Execute all 4 phases in order:

1. **Base Spec** -- Write `base.tla` + `base.cfg` with bug-family driven extensions
2. **MC Spec** -- Write `MC.tla` + `MC.cfg` with counter-bounded actions
3. **Trace Spec** -- Write `Trace.tla` + `Trace.cfg` for trace validation
4. **Instrumentation Spec** -- Write `instrumentation-spec.md` with action-to-code mapping

## Output

Create the output directory and write all files to:
  ${spec_dir}/

Expected files:
- `${spec_dir}/base.tla` -- Base specification
- `${spec_dir}/base.cfg` -- Base config
- `${spec_dir}/MC.tla` -- Model checking specification
- `${spec_dir}/MC.cfg` -- Model checking config
- `${spec_dir}/Trace.tla` -- Trace validation specification
- `${spec_dir}/Trace.cfg` -- Trace validation config
- `${spec_dir}/instrumentation-spec.md` -- Instrumentation mapping

## Critical Rules

1. Every extension traces to a Bug Family. No Bug Family reference = don't add the extension.
2. Model the implementation, not the paper. Deviations from the reference algorithm are where bugs live.
3. Follow the code's control flow faithfully. Do not simplify, reorder, or merge logic that the code keeps separate.
4. Annotate every logic block with source lines (file:line). Not optional.
5. Write to files early and often. Insurance against context loss.
6. Split actions where code paths diverge. Merging hides bugs.
7. Name actions after implementation functions. Enables cross-referencing with code.
8. Silent actions must be tightly constrained. Unconstrained silent actions cause state space explosion.
9. MC spec bounds fault-injection, not normal operations.
10. For Category B systems, split API-level operations at real semantic boundaries (read/confirm, reserve/publish, retire/reclaim, signal/complete). Do not collapse them into single actions unless the code is truly atomic there.
    \end{Verbatim}
\end{promptboxwithheader}

\begin{promptboxwithheader}{Phase 2 Agent Skill Prompt}
    \begin{Verbatim}[breaklines=true, breakanywhere=true]
# TLA+ Spec Generation

Bug-family driven modeling: each spec extension exists because a Bug Family in the Modeling Brief identified a concrete mechanism that needs verification. The spec logic within each action MUST faithfully follow the implementation's control flow, with every logic block annotated to its source code location.

## Input / Output

**Input**: `modeling-brief.md` + source code access

**Output** (written to files sequentially):

| Phase | Output | Description |
|-------|--------|-------------|
| 1 | `base.tla` + `base.cfg` | Base spec with all extensions |
| 2 | `MC.tla` + `MC.cfg` + `MC_hunt_*.cfg` | Model checking spec + hunting configs per bug family |
| 3 | `Trace.tla` + `Trace.cfg` | Trace validation spec |
| 4 | `instrumentation-spec.md` | Action-to-code mapping for harness generation |

**Single agent, sequential phases.** Each phase writes output to files. If context is compressed mid-session, re-read your own output files to recover.

---

## Step 0: Determine System Category

Before writing any spec files, read `modeling-brief.md` and determine whether the target is:

- **Category A (Distributed / Message-Passing)**
- **Category B (Concurrent / Lock-Free / Runtime)**

This should already be recorded in the brief. If it is missing, infer it from the source code and write the answer down before proceeding.

For **Category B** systems, do **not** force a message-passing template onto the code. The spec should usually center on:

- per-thread / per-task program counters
- cached snapshots vs current shared state
- linearization points
- memory-visibility bridges across variables
- retire / reclaim state
- ownership transfer and wakeup paths

---

## Phase 1: Base Spec

**Goal**: Write the core TLA+ specification with bug-family driven extensions.

1. **Read the Modeling Brief** -- note each Bug Family's mechanism, suggested variables/actions, priority
2. **Read source code (targeted)** -- only the functions referenced in the brief, not the entire codebase
3. **Design variables** -- standard protocol variables (Category A) or concurrency variables (Category B: thread-local snapshots, reclamation state, handoff flags, cached views) + extension variables motivated by Bug Families
4. **Write actions** -- name after implementation functions, follow code's control flow faithfully, annotate every logic block with `file:line`
5. **Write invariants** -- standard safety properties + extension invariants targeting Bug Families + structural invariants
6. **Write Init and Next**

**Read `references/base-spec-methodology.md`** for patterns, annotation style, and action design.

---

## Phase 2: MC Spec

**Goal**: Wrap the base spec with counter-bounded actions for exhaustive model checking.

Counter-bound fault-injection actions (timeout, crash, message loss, etc.). Do NOT bound deterministic/reactive actions. Add symmetry reduction, message buffer constraints, structural invariants, and temporal properties.

**Generate two types of config**:
- **`MC.cfg`** -- standard safety + structural invariants. Used during spec validation (convergence). Extension invariants (bug-family-specific) should be listed but **commented out**.
- **`MC_hunt_<family>.cfg`** -- one per bug family from the modeling brief. Tight bounds (reduce irrelevant actions to 0-1), only the target invariant + core safety invariants. Used during bug hunting after spec converges.

**Read `references/mc-spec-pattern.md`** for the full template and hunting config pattern.

---

## Phase 3: Trace Spec

**Goal**: Replay implementation traces against the base spec to verify consistency.

Key concepts: cursor variable `l` walks through trace events; action wrappers match events, call base actions, validate post-state, advance cursor; silent actions handle impl state changes without trace events (must be tightly constrained).

**ValidatePostState must be implemented, not a stub.** For each action wrapper, write field checks based on what `instrumentation-spec.md` defines as captured fields. The base spec tells you which variables each action modifies; the instrumentation spec tells you which fields will be in the trace. Match them. Do not leave `ValidatePostState == TRUE` -- Phase 2.5 and Phase 3 will reject it.

**Trace file location**: Trace files (`.ndjson`) are stored in `traces/` (sibling to `spec/`). The `JsonFile` operator in `Trace.tla` must default to `../traces/<name>.ndjson`, with an `IOEnv.JSON` override for per-run selection:
```tla
JsonFile ==
    IF "JSON" \in DOMAIN IOEnv THEN IOEnv.JSON
    ELSE "../traces/trace.ndjson"
```

**Read `references/trace-spec-pattern.md`** for the full template and silent action patterns.

---

## Phase 4: Instrumentation Spec

**Goal**: Produce a mapping document (`instrumentation-spec.md`) describing how to instrument the source code to produce traces compatible with the trace spec.

For each spec action, specify: spec action name, code location (`file:line`), trigger point (before/after which operation), and event fields to capture.

**Read `references/instrumentation-spec-format.md`** for the full format.

---

## Critical Rules

1. **Every extension traces to a Bug Family.** No Bug Family reference -> don't add the extension.
2. **Model the implementation, not the paper.** Deviations from the reference algorithm are where bugs live.
3. **Follow the code's control flow faithfully.** Do not simplify, reorder, or merge logic that the code keeps separate.
4. **Annotate every logic block with source lines.** Every condition, branch, and state update must cite `file:line`. Not optional.
5. **Write to files early and often.** Insurance against context loss.
6. **Split actions where code paths diverge.** Merging hides bugs.
7. **Name actions after implementation functions.** Enables cross-referencing with code.
8. **Silent actions must be tightly constrained.** Unconstrained silent actions cause state space explosion.
9. **MC spec bounds fault-injection, not normal operations.**
10. **For Category B, split operations at real semantic boundaries.** If code has separate read/confirm, reserve/publish, retire/reclaim, or signal/complete windows, do not collapse them into one action just because the public API looks atomic.

---

## Reference Files

- **`references/base-spec-methodology.md`** -- Variable design, action design, annotation style, invariants, helpers
- **`references/mc-spec-pattern.md`** -- MC spec template with counter-bounded actions
- **`references/trace-spec-pattern.md`** -- Trace spec template with event matching and silent actions
- **`references/instrumentation-spec-format.md`** -- Format for the action-to-code mapping document
- **`examples/hashicorp-raft-spec-generation.md`** -- Complete worked example

## Related Skills

- **code_analysis** -- Previous phase: produces the Modeling Brief
- **harness-generation** -- Next phase (2.5): instruments the system and collects traces using `instrumentation-spec.md`
- **validation-workflow** -- Phase 3: validates the spec using traces and model checking

## Additional References

For additional examples beyond the built-in ones, see the [Specula case-studies repository](https://github.com/specula-org/specula-case-studies) which contains 60+ completed case studies across distributed systems, consensus protocols, and concurrent data structures.
    \end{Verbatim}
\end{promptboxwithheader}

\subsection{Phase 3: Spec Refinement}
\label{app:prompts-phase3}
\begin{promptboxwithheader}{Phase 3 Launch Prompt}
    \begin{Verbatim}[breaklines=true, breakanywhere=true]
# Spec Validation Task: ${name}

You are validating the TLA+ specification for **${name}** through iterative trace validation and invariant checking.

## Inputs

- **Spec directory**: ${spec_dir}
  - base.tla, base.cfg -- Base specification
  - MC.tla, MC.cfg -- Model checking specification
  - Trace.tla, Trace.cfg -- Trace validation specification
  - instrumentation-spec.md -- Action-to-code mapping for harness generation
- **Source code**: ${repo_dir}
- **Modeling brief**: ${work_dir}/modeling-brief.md

## Workflow

Read and follow the **validation-workflow** skill:
  ${SPECULA_ROOT}/.claude/skills/validation-workflow/guide.md

This skill orchestrates the iterative loop between trace validation and model checking.
It delegates to two sub-skills (read these too):
  ${SPECULA_ROOT}/.claude/skills/tla-trace-workflow/guide.md
  ${SPECULA_ROOT}/.claude/skills/tla-checking-workflow/guide.md

Determine whether the target is Category A or Category B from `${work_dir}/modeling-brief.md`, the trace layout, and the instrumentation spec before debugging. Do not assume linear single-file traces for concurrent systems.

## Pre-step: Verify harness and traces

Harness and traces should already exist from Phase 2.5 (harness generation). Verify:
- Trace files in: ${work_dir}/traces/
- Instrumentation guide: ${work_dir}/harness/INSTRUMENTATION.md

If instrumentation adjustments are needed during validation, read `harness/INSTRUMENTATION.md` for how to modify capture points and fields, then re-run `bash harness/run.sh` to regenerate traces.

## Critical Rules

1. Follow the validation-workflow skill -- do not invent your own methodology.
2. The implementation is ground truth. When spec and implementation disagree, the spec is wrong (unless it's a real bug).
3. For Case C (real bug found): STOP and document it clearly. Do not "fix" real bugs.
4. For abstraction gaps: document them and make a pragmatic choice, then continue.
5. If the system is Category B, preserve the partial-order/timebox validation model. Do not "simplify" it into a linear trace workflow just to make validation easier.
    \end{Verbatim}
\end{promptboxwithheader}

\begin{promptboxwithheader}{Phase 3 Agent Skill Prompt}
    \begin{Verbatim}[breaklines=true, breakanywhere=true]
# TLA+ Verification Workflow (Orchestration)

Iteratively refine a TLA+ spec by alternating between trace validation and model checking until both pass, then hunt for real bugs using the converged spec. This ensures the spec faithfully models the system -- covering all real behaviors while excluding illegal states -- and then uses the trusted spec to find implementation bugs.

## Why Iteration is Necessary

- **Trace validation** ensures: spec covers all observed system behaviors (spec \supseteq system)
- **Model checking** ensures: spec doesn't allow illegal states (spec \subseteq legal states)

These pull in opposite directions. Fixing trace failures may loosen the spec (introducing illegal states). Fixing invariant violations may tighten the spec (breaking trace validation). Convergence happens when both pass simultaneously.

## Input

| Item | Description |
|------|-------------|
| Base spec | `base.tla` + `base.cfg` -- core specification |
| Trace spec | `Trace.tla` + `Trace.cfg` -- trace replay wrapper |
| MC spec | `MC.tla` + `MC.cfg` -- model checking wrapper (standard + structural invariants) |
| Hunting configs | `MC_hunt_*.cfg` / `MC_family*.cfg` -- bug-family-specific configs (for bug hunting) |
| Trace files | `.ndjson` files from instrumented test runs |
| Instrumentation spec | `instrumentation-spec.md` -- maps spec actions to source code locations |
| Run command | Command to launch TLC for model checking |

## Output

- Verified spec: all traces pass AND no invariant violations

### Required Artifacts

All artifacts are relative to `.specula-output/`:

| Artifact | Path | Description |
|----------|------|-------------|
| Changelog | `spec/changelog.md` | Unified record of all modifications across iterations (format below) |
| MC output | `spec/output/` | TLC model checking output files (counterexamples, statistics) |
| Bug report | `spec/bug-report.md` | Bug hunting results -- produced after convergence (even if no bugs found) |

---

## Phase 0: Initialization

1. **Verify all files exist**: base spec, trace spec, MC spec, trace files, instrumentation-spec, hunting configs
2. **Read `instrumentation-spec.md`**: understand the mapping between spec actions and source code locations -- you'll need this when analyzing failures and making fixes
3. **Read `harness/INSTRUMENTATION.md`**: understand how to adjust instrumentation if trace validation reveals capture timing or field issues
4. **Check `Trace.cfg` has `PROPERTIES TraceMatched`** (uncommented). If missing, add it -- without it validation reports false positives.
5. **Create `spec/changelog.md`** (or open existing one)

---

## Phase 1: Trace Validation Round

**Goal**: Ensure all traces pass validation.

**Delegate to sub-skill**: Follow the methodology in `../tla-trace-workflow/guide.md`.

**Steps**:
1. Run `run_trace_validation_parallel` on all trace files
2. For each failing trace: debug and fix following the trace workflow
3. After each fix, re-run `run_trace_validation_parallel` to check for regressions
4. Record each fix in `changelog.md` (see format below)
5. Continue until all traces pass

**When all traces pass**: proceed to Phase 2.

---

## Phase 2: Model Checking Round

**Goal**: Ensure no invariant violations in the spec's state space.

**Config**: Use **`MC.cfg` only** -- standard safety + structural invariants. Do NOT use hunting configs (`MC_hunt_*.cfg`) in this phase; those are for bug hunting after convergence.

**Run duration**: 30 minutes per run. See `../tla-checking-workflow/guide.md` Phase 1 "Runtime Parameters" for worker, memory, and simulation depth settings.

**Delegate to sub-skill**: Follow the methodology in `../tla-checking-workflow/guide.md`.

**Steps**:
1. Launch TLC model checking with `MC.cfg`
2. Monitor for violations
3. For each violation: analyze counterexample, classify (Case A/B/C), and fix following the checking workflow
4. Record each fix in `changelog.md`
5. **Case C (real bug)**: record as `[bug]` in changelog, save TLC output to `spec/output/`, then **continue** model checking -- do not stop convergence
6. After fixing Case A/B, restart model checking to verify fix and find more violations
7. Continue until model checking completes with no violations

**When model checking passes**: proceed to Phase 3.

---

## Phase 3: Convergence Check

**Decision logic**:

- If Phase 2 **modified the spec** -> go back to Phase 1 (spec changes may break trace validation)
- If Phase 2 **did not modify the spec** (only invariant changes or no changes) -> **converged**, proceed to Bug Hunting
- If Phase 1 **modified the spec** in a new round -> Phase 2 must re-run after

**Tracking regressions**: If a trace that passed in a previous round now fails, mark it as `[regression]` in changelog. This is informational -- handle it the same way as any other failure.

**Convergence**: Both phases pass in the same round with no spec modifications needed. The spec is now trusted. Proceed to Bug Hunting.

---

## Bug Hunting

**Precondition**: Spec has converged (Phase 3 passed). The spec is trusted to faithfully model the implementation.

**Goal**: Use the converged spec to find real implementation bugs via targeted model checking with bug-family configs.

### BFS + Simulation Strategy

For each hunting config, alternate between BFS and simulation to maximize coverage:

1. **BFS first** (30 min) -- exhaustive within reachable diameter. Check the diameter achieved in TLC output.
2. **If diameter <= 25** -- the BFS run is too shallow to expose many bugs. Follow up with a **simulation run** (30 min) on the same config to reach deeper states.
3. **If diameter > 25** -- BFS coverage is likely sufficient. Simulation follow-up is optional.

**Do NOT shrink config bounds to make BFS go deeper.** Counter bounds (timeout limits, crash limits, etc.) directly control which bug scenarios are reachable. Reducing them to fit BFS eliminates the very interleavings where bugs hide. When BFS is too shallow, use simulation for depth -- not tighter bounds.

### Steps

1. Collect any `[bug]` entries already recorded in `changelog.md` during Phase 2 (Case C found during convergence) -- these will be included in the final report
2. For each `MC_hunt_*.cfg` / `MC_family*.cfg`:
   - **Run 1 (BFS)**: Launch TLC model checking (30 min). Record diameter and state count from output.
   - If violation found -> **Case C** (real bug). Analyze counterexample: describe execution path, cross-reference with implementation code, identify root cause and affected code locations.
   - If no violation and diameter <= 25 -> **Run 2 (Simulation)**: Launch TLC simulation (30 min, `-S -n 999999999`) on the same config for deeper exploration.
   - Save all TLC output to `spec/output/`
3. Produce `spec/bug-report.md` with all findings -- **read `references/bug-report-format.md`** for the template
4. If no bugs found across all configs: still write the report (state space coverage, diameter achieved per config, + "no violations found")

---

## changelog.md Format

Maintain a single `spec/changelog.md`. One line per fix, grouped by round.

```markdown
## Round N - Trace Validation
- [fix] ActionName: brief description of what was wrong and how it was fixed (Trace: filename.ndjson)
- [regression] ActionName: brief description (Trace: filename.ndjson, was passing in Round M)

## Round N - Model Checking
- [fix-inv] InvariantName: brief description of invariant change (Case A)
- [fix-spec] ActionName: brief description of spec change (Case B)
- [bug] ActionName: brief description of real bug found (Case C)

## Result
Converged in N rounds. Bug hunting: M bugs found / no bugs found.
```

**Keep entries concise** -- a few sentences per fix is enough.

---

## Critical Rules

1. **Always start with trace validation.** Ensure spec covers real behavior first, then tighten.
2. **Complete each phase fully before switching.** Don't interleave -- finish all traces, then finish model checking.
3. **Delegate to sub-skills.** This layer decides WHAT to run; sub-skills decide HOW to debug and fix.
4. **Record every fix in changelog.** This is the single source of truth for the iteration history.
5. **Autonomous by default.** Apply fixes directly. Only pause for user confirmation if the prompt explicitly requests human-in-the-loop.
6. **Read instrumentation-spec before fixing.** Always know the code location mapping when analyzing failures.

---

## Sub-Skills

- **`../tla-trace-workflow/guide.md`** -- Trace validation: validate, debug, fix
- **`../tla-checking-workflow/guide.md`** -- Model checking: run, analyze counterexamples, fix

## Related Skills

- **harness-generation** -- Previous phase (2.5): produces harness, traces, and `INSTRUMENTATION.md` for adjusting instrumentation during validation
- **spec-generation** -- Produces the TLA+ specs that this workflow verifies
- **code-analysis** -- Analyzes system implementation to produce modeling briefs

## Additional References

For additional examples beyond the built-in ones, see the [Specula case-studies repository](https://github.com/specula-org/specula-case-studies) which contains 60+ completed case studies across distributed systems, consensus protocols, and concurrent data structures.
    \end{Verbatim}
\end{promptboxwithheader}

\subsection{Phase 4: Bug Confirmation}
\label{app:prompts-phase4}
\begin{promptboxwithheader}{Phase 4 Launch Prompt}
    \begin{Verbatim}[breaklines=true, breakanywhere=true]
# Bug Confirmation Task: ${name}

You are confirming and reproducing bugs found in **${name}** by both model checking and code review.

## Inputs

- **Bug report (MC findings)**: ${spec_dir}/bug-report.md
- **Modeling brief (code review findings)**: ${work_dir}/modeling-brief.md
- **Source code**: ${repo_dir}
- **Spec directory**: ${spec_dir}

## Methodology

Read and follow the **bug-confirmation** skill:
  ${SPECULA_ROOT}/.claude/skills/bug-confirmation/guide.md

## Task

### Step 1: Consolidate all findings

Read both `bug-report.md` (MC-confirmed bugs) and `modeling-brief.md` (code review findings).
Create a unified list of all bugs/findings, noting for each:
- Source: MC (with counterexample) or code review
- Severity assessment
- Affected code location

Filter out defensive coding suggestions, style issues, and theoretical-only concerns.
Keep only findings that represent real logic bugs with concrete impact.

### Step 2: Confirm each bug via code audit

For each finding, follow the bug-confirmation skill Phase 1:
1. Locate and read the relevant code in the source repo
2. Trace the call chain -- is the buggy path reachable?
3. Check for existing safeguards that prevent the bug
4. Construct a concrete trigger scenario

Classify each finding as:
- **CONFIRMED**: Code audit confirms the bug is real and reachable
- **FALSE POSITIVE**: Safeguards exist that prevent the bug in practice
- **NEEDS REPRODUCTION**: Bug is plausible but needs a test to verify

### Step 3: MANDATORY -- Reproduce every confirmed bug

**This step is NOT optional.** Every bug classified as CONFIRMED or NEEDS REPRODUCTION MUST have a reproduction test. A bug without reproduction is NOT confirmed -- it is unverified.

For each confirmed bug:
1. Write a self-contained reproduction test to `${work_dir}/repro/`
2. The test MUST use the system's public interfaces -- no illegal state injection
3. The test MUST actually be executed, and the output recorded
4. For concurrency bugs: real multi-thread/multi-process scenarios. Small delays (sleep, failpoints) to widen race windows are OK, but the logic must not be altered.
5. For distributed systems: use Docker or the system's test framework to set up a real cluster
6. Success criterion: observable anomalous behavior (crash, deadlock, data inconsistency, invariant violation)
7. If reproduction fails after genuine effort: explain what was tried, why it failed, and whether the bug is still believed to be real. Do NOT silently skip reproduction.

**Output requirement**: At least one executable file in `${work_dir}/repro/` for each confirmed bug. Name them `test_bug1_*.py`, `test_bug2_*.py`, etc.

### Step 4: Write final report

Write the final consolidated report to: ${spec_dir}/confirmed-bugs.md

Format:
```markdown
# Confirmed Bug Report -- ${name}

## Summary
- Total findings reviewed: N
- Reproduced: N
- Confirmed (code audit, reproduction failed): N
- False positives: N
- Inconclusive: N

## Bug 1: <title>
- **Source**: MC / Code Review
- **Status**: REPRODUCED / REPRODUCTION FAILED / FALSE POSITIVE
- **Severity**: Critical / High / Medium
- **Location**: file:line
- **Description**: ...
- **Trigger scenario**: ...
- **Reproduction test**: repro/test_bug1_xxx.py -- describe what it does
- **Reproduction result**: PASS (bug triggered) / FAIL (bug not triggered, explain why)
- **Recommendation**: ...
```

## Critical Rules

1. Follow the bug-confirmation skill strictly -- especially the prohibited approaches.
2. **Every confirmed bug MUST have a reproduction test in repro/.** No exceptions. "Code audit only" is NOT an acceptable final status for new bugs.
3. MC-confirmed bugs with counterexamples are high-confidence; focus reproduction effort there first.
4. Do NOT lower reproduction standards to claim success. If you cannot reproduce, say so honestly -- but you MUST try.
5. For each false positive, explain clearly what safeguard prevents the bug.
6. Actually RUN the reproduction tests and record the output. Do not just write tests without executing them.
    \end{Verbatim}
\end{promptboxwithheader}

\begin{promptboxwithheader}{Phase 4 Agent Skill Prompt}
    \begin{Verbatim}[breaklines=true, breakanywhere=true]
## Bug Confirmation and Reproduction Guide

### Phase 1: Code Audit

Before attempting reproduction, you **must** first confirm the bug's validity by reading the source code.

1. **Locate the relevant code**: Find the specific functions and lines mentioned in the bug report. Read these functions in full and understand their context.
2. **Trace the call chain**: Starting from public APIs or entry points, trace the path to the buggy code. Confirm whether this path is reachable during normal usage.
3. **Check for existing safeguards**: Check whether callers already have precondition checks, lock guards, or other mechanisms that prevent this bug from being triggered in practice. If they do, the bug is a false positive -- report it and stop.
4. **Construct a trigger scenario**: Describe in words a concrete sequence of events that could naturally occur at the user/system level and would reach the buggy code path. If you cannot construct one, the bug is likely a false positive.

Only proceed to Phase 1.5 after completing the above steps and being confident the code path is reachable.

### Phase 1.5: Developer Intent Investigation

A bug is defined by the developers' own requirements and expectations -- not by the researcher's intuition about what should be correct. Before investing effort in reproduction, investigate what the developers themselves believe about this behavior.

**What to investigate:**

1. **Issue tracker**: Search for open and closed issues, PRs, and discussions mentioning the relevant code, function names, or the behavior in question. Developers may have already discussed this exact scenario.
2. **Commit messages and PR discussions**: Use `git log` and `git blame` on the affected code. Read the commit messages and linked PRs to understand why the code was written this way. Look for statements of intent ("this is a trade-off", "we accept this because...", "this should be safe even if...").
3. **Code comments and documentation**: Look for comments near the code (TODOs, FIXMEs, "known issue", "by design", "trade-off"), as well as design documents, RFCs, or architecture docs in the repository.
4. **Test cases**: Check what the existing tests assert. Tests encode developer expectations -- if a test explicitly sets up the scenario you found and asserts the current behavior, the developers likely consider it correct.

**How to use what you find:**

- **Developer says "we know about this, it's a deliberate trade-off"** -> Classify as NOT a bug unless you can show their trade-off analysis is flawed (e.g., they accepted a liveness cost but didn't realize it also affects safety).
- **Developer says "this should be safe even under condition X"** -> If your counterexample shows it is NOT safe under condition X, this IS a bug -- the developers' own stated requirement is violated.
- **No developer commentary found** -> Fall back to code quality analysis: assess whether the behavior constitutes a bug based on established engineering standards (e.g., violating API contracts, ignoring error returns, TOCTOU races, missing atomicity). These are bugs by any reasonable standard regardless of developer intent. Note the absence of developer evidence in your report and explain which engineering principle the code violates.

The two symmetric cases above are the key insight: developer intent can both _dismiss_ a finding that looks like a bug to a researcher, and _validate_ a finding that a researcher would have dismissed. Always let the evidence speak.

**Report what you find**: Whether the investigation confirms or refutes the bug, include a brief summary of the developer evidence in your final report. This makes the finding credible and actionable.

Only proceed to Phase 2 after completing the above steps and being confident the bug is real and that developers would consider it a bug.

### Phase 2: Low-Invasiveness Reproduction (MANDATORY for new bugs)

**Phase 2 is MANDATORY for every NEW bug** -- i.e., bugs that do not correspond to an existing JIRA ticket, CVE, or previously reported issue. A new bug without a reproduction test is unverified speculation, not a confirmed finding.

**Known/historical bugs** (those matching an existing JIRA ticket) do NOT require reproduction -- the existing ticket serves as confirmation. Classify them and move on.

**For every new bug, you MUST**:
1. Write a self-contained reproduction test to `repro/test_bug<N>_<name>.py` (or `.js`, `.rs`, `.go` etc.)
2. Actually EXECUTE the test and record the output
3. Report the result honestly: REPRODUCED (bug triggered) or REPRODUCTION FAILED (bug not triggered, explain why)

"Code audit only" is NOT an acceptable final status for new bugs. If you skip reproduction for a new bug, the finding is considered unverified.

The core principle: **simulate a real-world trigger, not bypass normal flows to poke the bug directly.**

**Prohibited approaches:**
- Pre-populating data structures with illegal or inconsistent state, then calling a function to "prove" it can't handle it
- Directly calling internal/private functions, skipping normal entry-point checks
- Manually constructing inputs that could never occur through normal flows
- Modifying the code under test to create the bug (e.g., commenting out validation logic)

**Correct approaches:**
- Trigger through the system's public interfaces or normal entry points
- For concurrency bugs, reproduce via real concurrent scenarios (multi-thread/multi-process). Small delays may be inserted into the code under test to widen the race window, but the logic must not be altered
- For protocol bugs, trigger via sequences of messages that are legitimate but adversarial. The messages themselves must pass the system's normal validation
- The reproduction program should compile and run independently, without requiring special environments beyond the test framework
- The success criterion must be observable anomalous behavior (crash, deadlock, data inconsistency, safety property violation), not "some intermediate variable has an unexpected value"

**Criteria for successful reproduction:**
- The bug is triggered without modifying the core logic of the system under test
- The trigger path is consistent with real-world usage scenarios
- The reproduction is deterministic, or triggers with significant probability across multiple runs
- The erroneous behavior caused by the bug is clearly observable

**Escalation ladder -- start low-invasiveness, escalate if needed:**

Your goal is to either **prove the bug exists** (trigger it) or **prove it doesn't** (explain why it's impossible to trigger). You must reach one of these conclusions. "I tried once and it didn't trigger" is NOT a conclusion.

1. **Level 0 -- Pure black-box**: Use only public APIs, normal operations, no failpoints. Try this first.
2. **Level 1 -- Timing assistance**: Add `sleep()` calls or use system-provided test hooks (e.g., `configureFailPoint`, `FAIL_POINT_DEFINE`) to widen race windows. The system logic is unchanged; you're only controlling timing.
3. **Level 2 -- State injection**: Directly inject the pre-condition state (e.g., insert a document that mimics a crash-recovery scenario) and verify the buggy code path handles it incorrectly. Clearly document that this is a state-injection test, not an end-to-end trigger.
4. **Level 3 -- Minimal code modification**: Add a small delay (`usleep`, `sleep`) inside the system's source code at the exact crash window location to make the race deterministic. Document the modification precisely.

Start at Level 0. If it doesn't trigger, analyze WHY (what timing/state condition is missing?), then escalate to the next level. Each escalation must be explained. **Do not stop at Level 0 failure.**

**Verify you triggered the RIGHT bug:**

After triggering anomalous behavior, verify it matches the MC counterexample. Compare:
- The sequence of operations matches the MC trace (same actions, same order)
- The violated invariant is the same one MC found
- The root cause is the same code path MC identified

If you triggered a DIFFERENT bug than what MC found, report it separately but continue trying to trigger the original MC bug.

**Evidence requirements:**

When reporting REPRODUCED, you MUST include:
- The exact command used to run the test
- The actual output (copy-paste from terminal, not paraphrased)
- Which line(s) of output demonstrate the bug was triggered
- Comparison with expected (correct) behavior

When reporting REPRODUCTION FAILED after exhausting the escalation ladder:
- Which levels you attempted (0 through 3)
- For each level: what you tried, what happened, why it didn't trigger
- Your conclusion: is the bug real but hard to trigger, or is it a false positive?

**If reproduction fails:**
- Explain what approaches were attempted at each escalation level and why they failed
- Analyze whether the bug itself is a false positive, or whether the trigger conditions are difficult to satisfy in the current test environment
- Do not lower the bar of reproduction authenticity just to claim "reproduction succeeded"
- The reproduction test file MUST still exist in `repro/` with the failed attempt code and a comment explaining why it didn't trigger

**Output requirements (non-negotiable for new bugs):**
- For each NEW confirmed bug: one executable test file in `repro/test_bug<N>_*.{py,js,rs,go,c,sh}`
- The test must have been actually executed (not just written)
- The confirmed-bugs.md must include **actual test output** (copy-paste) as evidence, not just a status label
- If new bugs exist but zero reproduction tests exist, the confirmation is INVALID
- Known/historical bugs do not require reproduction files

## Additional References

For additional examples beyond the built-in ones, see the [Specula case-studies repository](https://github.com/specula-org/specula-case-studies) which contains 60+ completed case studies across distributed systems, consensus protocols, and concurrent data structures.
    \end{Verbatim}
\end{promptboxwithheader}
