# Supplementary material for: Specula: Scaling formal specifications for autonomous model checking of system code
Source: arXiv:2607.25333 source file (2026-08-03)
Supplement: Supplementary file 6 [file 10_cost_time_full.tex]

\section{Per-Module Cost and Runtime}
\label{app:rq3-cost-time}

\toreview{%
Table~\ref{tab:app-cost-time-full} reports the per-module cost and runtime behind
    \S\ref{sec:eval-resources} for the five controlled experiment systems
    (\S\ref{sec:eval-baselines}).}

\begin{table*}[t]
\centering
\caption{\toreview{Per-module token cost (USD) and runtime (minutes) for the five
  controlled experiment systems. Agent-Raw and Agent-\tla{} are the two baselines;
  \specula is split by phase (P1--P4), with the per-run total (\textbf{Tot}). The last row is
  the per-column mean.}}
\label{tab:app-cost-time-full}
\resizebox{\textwidth}{!}{%
\setlength{\tabcolsep}{4pt}
\begin{tabular}{l l rr rr rrrrr rrrrr}
\toprule
& & \multicolumn{2}{c}{Agent-Raw} & \multicolumn{2}{c}{Agent-\tla{}}
  & \multicolumn{5}{c}{\specula cost (\$)} & \multicolumn{5}{c}{\specula time (min)} \\
\cmidrule(lr){3-4}\cmidrule(lr){5-6}\cmidrule(lr){7-11}\cmidrule(lr){12-16}
\textbf{System} & \textbf{Module} & min & \$ & min & \$
  & P1 & P2 & P3 & P4 & \textbf{Tot}
  & P1 & P2 & P3 & P4 & \textbf{Tot} \\
\midrule
Autobahn   & ---       & 27.4 & 5.99 & 68.9 & 16.46 &  6.11 &  8.43 &  4.79 &  9.63 &  28.96 & 17 &  38 &  32 & 23 & 110 \\
\midrule
CometBFT   & ---       & 40.1 & 6.27 & 13.0 &  2.58 & 18.66 & 35.72 & 98.17 & 15.28 & 167.83 & 27 & 115 & 232 & 28 & 402 \\
\midrule
sofa-jraft & ---       & 11.0 & 2.19 & 24.4 &  4.91 & 13.32 & 47.55 & 11.19 &  9.00 &  81.06 & 17 & 111 &  37 & 34 & 199 \\
\midrule
\multirow{5}{*}{MongoDB}
  & chunkmigration           & 12.5 & 3.71 & 14.6 & 4.47 & 19.48 & 14.34 &  3.84 &  7.80 & 45.46 & 38 &  56 & 11 & 43 & 148 \\
  & rangedeletion            & 20.7 & 5.07 & 18.4 & 5.59 &  9.52 & 14.90 &  3.97 &  5.03 & 33.42 & 19 &  64 & 14 & 31 & 128 \\
  & rangedeletions-secondary & 18.5 & 4.58 & 12.9 & 3.74 & 19.80 & 13.19 &  3.09 &  6.16 & 42.24 & 30 &  94 & 12 & 30 & 166 \\
  & session                  & 10.8 & 2.84 & 10.8 & 3.36 & 15.72 & 16.97 &  4.70 &  3.49 & 40.88 & 29 &  71 & 18 & 16 & 134 \\
  & raftreconfig             & 12.6 & 2.88 & 20.4 & 4.15 & 10.75 & 41.92 & 12.01 & 11.04 & 75.72 & 27 & 105 & 37 & 41 & 210 \\
\midrule
\multirow{11}{*}{libspdm}
  & cert-auth         &  7.7 & 2.21 & 13.3 & 3.84 & 12.19 & 25.82 & 14.13 &  7.92 & 60.06 & 23 & 121 & 247 & 29 & 420 \\
  & chunking          & 13.8 & 3.22 & 15.5 & 4.31 &  6.65 & 13.20 &  3.19 &  6.17 & 29.21 & 14 &  47 &  17 & 17 &  95 \\
  & events            & 14.8 & 4.54 & 12.6 & 4.06 &  9.18 & 12.44 &  4.90 &  4.01 & 30.53 & 29 &  43 &  18 & 12 & 102 \\
  & key-exchange      &  8.6 & 2.87 & 14.5 & 5.81 & 10.15 & 29.92 &  4.93 &  7.30 & 52.30 & 13 & 107 &  48 & 21 & 189 \\
  & meas-ext-log      & 10.5 & 2.36 & 15.3 & 4.29 &  5.74 & 23.63 &  8.96 &  5.72 & 44.05 & 18 &  44 &  39 & 12 & 113 \\
  & measurements      & 12.6 & 4.25 &  8.4 & 3.21 &  9.06 & 18.38 &  3.67 &  9.68 & 40.79 & 16 &  53 &  15 & 30 & 114 \\
  & mut-auth-encap    & 12.8 & 3.42 & 15.1 & 4.27 &  7.61 &  5.81 &  5.31 &  4.33 & 23.06 & 18 &  24 &  11 & 16 &  69 \\
  & psk-exchange      &  9.4 & 2.90 & 19.4 & 6.28 &  8.82 & 21.06 &  4.19 &  3.60 & 37.67 & 19 &  59 &  16 & 13 & 107 \\
  & secured-message   & 28.9 & 7.13 & 22.9 & 7.84 &  7.23 & 19.44 &  3.43 &  3.56 & 33.66 & 15 &  85 &  12 & 16 & 128 \\
  & session-lifecycle & 20.6 & 5.16 & 15.0 & 4.87 &  3.53 & 19.27 &  8.05 &  5.72 & 36.57 & 13 &  87 &  45 & 15 & 160 \\
  & version-cap-algo  & 13.7 & 3.84 & 19.6 & 7.15 &  8.09 & 30.55 &  8.45 & 13.22 & 60.31 & 16 & 116 &  16 & 17 & 165 \\
\midrule
\multicolumn{2}{l}{\textbf{Mean}}
  & 16.2 & 3.97 & 18.7 & 5.33 & 10.61 & 21.71 & 11.10 & 7.30 & \textbf{50.73}
  & 21 & 76 & 46 & 23 & \textbf{166} \\
\bottomrule
\end{tabular}}
\end{table*}
