# Supplementary material for: Specula: Scaling formal specifications for autonomous model checking of system code
Source: arXiv:2607.25333 source file (2026-08-03)
Supplement: Supplementary file 7 [file 11_rq5_models.tex]

\section{Per-Module Results Across Agents}
\label{app:rq5-models}
\label{app:rq3-cost-time}

\toreview{%
This appendix reports per-module results for all five configurations behind
    \S\ref{sec:eval-baselines}--\S\ref{sec:eval-models}: the two baselines
    (Agent-Raw, Agent-\tla{}) and \specula{} under Opus, Sonnet, and Haiku.
    Tables~\ref{tab:app-bugs}--\ref{tab:app-time} give bugs, cost, and runtime,
    Table~\ref{tab:app-sysmobench} gives SysMoBench specification quality scores, and
    Tables~\ref{tab:app-phase-opus}--\ref{tab:app-phase-haiku} break each \specula{}
    run's cost and runtime down by pipeline phase. Bug counts are ground-truth hits,
    with each agent's false positives totaled in the bottom rows of
    Table~\ref{tab:app-bugs}. Runtime is reported as active
    compute time, with the idle between phases (for example, API rate-limit waits)
    excluded, so the whole-run figures in Table~\ref{tab:app-time} equal the per-phase
    sums in Tables~\ref{tab:app-phase-opus}--\ref{tab:app-phase-haiku}.%
}

\toreview{%
Table~\ref{tab:app-sysmobench} scores every specification the five agents produced on the
    four SysMoBench metrics~\cite{cheng2026sysmobench}: syntax validation (the
    fraction of \tla{} actions with valid syntax), model checking (the fraction of
    actions TLC can execute), conformance (the fraction of implementation actions
    that trace validation replays on the model without error), and invariant
    correctness (the fraction of the benchmark's template invariants that hold on
    the model).%
}

\begin{table*}[t]
\centering
\small
\setlength{\tabcolsep}{6pt}
\caption{\toreview{Per-module bug counts (ground-truth hits) for all five agents, with each agent's total ground-truth hits and false positives in the bottom rows.}}
\label{tab:app-bugs}
\begin{tabular}{ll ccccc}
\toprule
\textbf{System} & \textbf{Module} & Agent-Raw & Agent-\tla{} & Opus & Sonnet & Haiku \\
\midrule
Autobahn & BFT consensus & 1 & 1 & 16 & 4 & 0 \\
\midrule
CometBFT & PBTS & 0 & 0 & 11 & 2 & 0 \\
\midrule
\multirow{11}{*}{libspdm} & cert auth & 0 & 0 & 1 & 0 & 0 \\
 & chunking & 0 & 0 & 2 & 0 & 0 \\
 & events & 0 & 0 & 4 & 1 & 0 \\
 & key exchange & 0 & 1 & 1 & 0 & 0 \\
 & measurement log & 0 & 0 & 3 & 2 & 0 \\
 & measurements & 0 & 1 & 2 & 1 & 0 \\
 & mutual auth & 0 & 0 & 0 & 0 & 0 \\
 & PSK exchange & 0 & 0 & 0 & 0 & 0 \\
 & secured messages & 0 & 0 & 0 & 0 & 0 \\
 & session lifecycle & 1 & 0 & 3 & 0 & 0 \\
 & version negotiation & 0 & 0 & 1 & 0 & 0 \\
\midrule
\multirow{5}{*}{MongoDB} & chunk migration & 0 & 0 & 4 & 0 & 0 \\
 & Raft reconfig & 0 & 0 & 0 & 0 & 0 \\
 & range deletion & 0 & 0 & 1 & 0 & 0 \\
 & range preservation & 0 & 0 & 2 & 0 & 0 \\
 & sessions & 0 & 0 & 1 & 0 & 0 \\
\midrule
sofa-jraft & Raft & 0 & 0 & 10 & 0 & 0 \\
\midrule
\multicolumn{2}{l}{\textbf{Total GT}} & 2 & 3 & 62 & 10 & 0 \\
\multicolumn{2}{l}{\textbf{False positives}} & 5 & 2 & 0 & 6 & 0 \\
\bottomrule
\end{tabular}
\end{table*}

\begin{table*}[t]
\centering
\small
\setlength{\tabcolsep}{6pt}
\caption{\toreview{Per-module token cost (USD) for all five agents.}}
\label{tab:app-cost}
\begin{tabular}{ll rrrrr}
\toprule
\textbf{System} & \textbf{Module} & Agent-Raw & Agent-\tla{} & Opus & Sonnet & Haiku \\
\midrule
Autobahn & BFT consensus & 5.99 & 16.46 & 28.96 & 36.37 & 2.53 \\
\midrule
CometBFT & PBTS & 6.27 & 2.58 & 167.83 & 32.78 & 2.38 \\
\midrule
\multirow{11}{*}{libspdm} & cert auth & 2.21 & 3.84 & 60.06 & 30.59 & 3.09 \\
 & chunking & 3.22 & 4.31 & 29.21 & 31.88 & 2.54 \\
 & events & 4.54 & 4.06 & 30.53 & 26.50 & 2.73 \\
 & key exchange & 2.87 & 5.81 & 52.30 & 31.58 & 2.89 \\
 & measurement log & 2.36 & 4.29 & 44.05 & 35.72 & 3.06 \\
 & measurements & 4.25 & 3.21 & 40.79 & 44.05 & 2.65 \\
 & mutual auth & 3.42 & 4.27 & 23.06 & 33.34 & 2.53 \\
 & PSK exchange & 2.90 & 6.28 & 37.67 & 32.96 & 3.15 \\
 & secured messages & 7.13 & 7.84 & 33.66 & 47.54 & 3.67 \\
 & session lifecycle & 5.16 & 4.87 & 36.57 & 21.66 & 3.00 \\
 & version negotiation & 3.84 & 7.15 & 60.31 & 28.34 & 3.35 \\
\midrule
\multirow{5}{*}{MongoDB} & chunk migration & 3.71 & 4.47 & 45.46 & 25.18 & 1.39 \\
 & Raft reconfig & 2.88 & 4.15 & 75.72 & 43.30 & 3.52 \\
 & range deletion & 5.07 & 5.59 & 33.42 & 22.42 & 2.57 \\
 & range preservation & 4.58 & 3.74 & 42.24 & 15.25 & 2.30 \\
 & sessions & 2.84 & 3.36 & 40.88 & 23.28 & 5.78 \\
\midrule
sofa-jraft & Raft & 2.19 & 4.91 & 81.06 & 29.06 & 3.33 \\
\midrule
\multicolumn{2}{l}{\textbf{Mean}} & 3.97 & 5.33 & 50.73 & 31.15 & 2.97 \\
\bottomrule
\end{tabular}
\end{table*}

\begin{table*}[t]
\centering
\small
\setlength{\tabcolsep}{6pt}
\caption{\toreview{Per-module runtime (minutes) for all five agents. Runtime is active compute time: the per-phase agent durations summed, with the idle between phases (for example, waiting on API rate limits) excluded. The whole-run total therefore equals the per-phase sum in Tables~\ref{tab:app-phase-opus}--\ref{tab:app-phase-haiku}.}}
\label{tab:app-time}
\begin{tabular}{ll rrrrr}
\toprule
\textbf{System} & \textbf{Module} & Agent-Raw & Agent-\tla{} & Opus & Sonnet & Haiku \\
\midrule
Autobahn & BFT consensus & 27 & 69 & 110 & 193 & 23 \\
\midrule
CometBFT & PBTS & 40 & 13 & 402 & 224 & 28 \\
\midrule
\multirow{11}{*}{libspdm} & cert auth & 8 & 13 & 420 & 150 & 38 \\
 & chunking & 14 & 16 & 95 & 226 & 24 \\
 & events & 15 & 13 & 102 & 128 & 28 \\
 & key exchange & 9 & 14 & 189 & 162 & 24 \\
 & measurement log & 10 & 15 & 113 & 194 & 29 \\
 & measurements & 13 & 8 & 114 & 288 & 32 \\
 & mutual auth & 13 & 15 & 69 & 179 & 26 \\
 & PSK exchange & 9 & 19 & 107 & 189 & 31 \\
 & secured messages & 29 & 23 & 128 & 231 & 33 \\
 & session lifecycle & 21 & 15 & 160 & 152 & 31 \\
 & version negotiation & 14 & 20 & 165 & 222 & 27 \\
\midrule
\multirow{5}{*}{MongoDB} & chunk migration & 12 & 15 & 148 & 166 & 18 \\
 & Raft reconfig & 13 & 20 & 210 & 249 & 33 \\
 & range deletion & 21 & 18 & 128 & 119 & 28 \\
 & range preservation & 18 & 13 & 166 & 103 & 26 \\
 & sessions & 11 & 11 & 134 & 209 & 52 \\
\midrule
sofa-jraft & Raft & 11 & 24 & 199 & 180 & 38 \\
\midrule
\multicolumn{2}{l}{\textbf{Mean}} & 16 & 19 & 166 & 188 & 30 \\
\bottomrule
\end{tabular}
\end{table*}

\begin{table*}[t]
\centering
\scriptsize
\setlength{\tabcolsep}{5pt}
\caption{\toreview{SysMoBench specification quality scores per module for all five agents~\cite{cheng2026sysmobench}. Syn.\ = syntax validation, MC = model checking, Conf.\ = conformance, Inv.\ = invariant correctness, Ovr.\ = the weighted overall $0.15\,\text{Syn} + 0.15\,\text{MC} + 0.35\,\text{Conf} + 0.35\,\text{Inv}$.}}
\label{tab:app-sysmobench}
\begin{tabular}{lrrrrr @{\hskip 18pt} lrrrrr}
\toprule
 & Syn. & MC & Conf. & Inv. & Ovr. & & Syn. & MC & Conf. & Inv. & Ovr. \\
\midrule
\multicolumn{6}{l}{\textbf{Autobahn}} & \multicolumn{6}{l}{\textbf{libspdm / secured messages}} \\
\quad Agent-Raw & \excellentcell{}100\% & \excellentcell{}100\% & \excellentcell{}83\% & \excellentcell{}100\% & \excellentcell{}94\% & \quad Agent-Raw & \excellentcell{}100\% & \goodcell{}67\% & \goodcell{}67\% & \excellentcell{}100\% & \excellentcell{}83\% \\
\quad Agent-\tla{} & \excellentcell{}100\% & \excellentcell{}83\% & \excellentcell{}83\% & \goodcell{}67\% & \excellentcell{}80\% & \quad Agent-\tla{} & \excellentcell{}100\% & \goodcell{}67\% & \goodcell{}67\% & \excellentcell{}100\% & \excellentcell{}83\% \\
\quad Opus & \excellentcell{}100\% & \excellentcell{}100\% & \excellentcell{}100\% & \excellentcell{}100\% & \excellentcell{}100\% & \quad Opus & \excellentcell{}100\% & \excellentcell{}100\% & \excellentcell{}100\% & \excellentcell{}100\% & \excellentcell{}100\% \\
\quad Sonnet & \excellentcell{}100\% & \excellentcell{}100\% & \excellentcell{}83\% & \goodcell{}71\% & \excellentcell{}84\% & \quad Sonnet & \excellentcell{}100\% & \excellentcell{}100\% & \excellentcell{}100\% & \goodcell{}67\% & \excellentcell{}88\% \\
\quad Haiku & \excellentcell{}100\% & \faircell{}33\% & \faircell{}17\% & 0\% & \faircell{}26\% & \quad Haiku & \excellentcell{}100\% & \excellentcell{}83\% & \faircell{}33\% & \goodcell{}67\% & \goodcell{}63\% \\
\addlinespace[2pt]
\multicolumn{6}{l}{\textbf{CometBFT}} & \multicolumn{6}{l}{\textbf{libspdm / session lifecycle}} \\
\quad Agent-Raw & \excellentcell{}100\% & \excellentcell{}83\% & \goodcell{}67\% & \excellentcell{}100\% & \excellentcell{}86\% & \quad Agent-Raw & \excellentcell{}100\% & \excellentcell{}100\% & \excellentcell{}100\% & \excellentcell{}86\% & \excellentcell{}95\% \\
\quad Agent-\tla{} & \excellentcell{}100\% & \excellentcell{}83\% & \excellentcell{}83\% & \excellentcell{}100\% & \excellentcell{}92\% & \quad Agent-\tla{} & \excellentcell{}100\% & \excellentcell{}83\% & \excellentcell{}83\% & \excellentcell{}88\% & \excellentcell{}87\% \\
\quad Opus & \excellentcell{}100\% & \excellentcell{}100\% & \excellentcell{}100\% & \excellentcell{}100\% & \excellentcell{}100\% & \quad Opus & \excellentcell{}100\% & \excellentcell{}100\% & \excellentcell{}100\% & \excellentcell{}100\% & \excellentcell{}100\% \\
\quad Sonnet & \excellentcell{}100\% & \excellentcell{}100\% & \excellentcell{}100\% & \excellentcell{}100\% & \excellentcell{}100\% & \quad Sonnet & \excellentcell{}100\% & \excellentcell{}100\% & \excellentcell{}100\% & \excellentcell{}88\% & \excellentcell{}96\% \\
\quad Haiku & \excellentcell{}100\% & \goodcell{}67\% & \faircell{}33\% & 0\% & \faircell{}37\% & \quad Haiku & \excellentcell{}100\% & \excellentcell{}100\% & \excellentcell{}83\% & 0\% & \goodcell{}59\% \\
\addlinespace[2pt]
\multicolumn{6}{l}{\textbf{libspdm / cert auth}} & \multicolumn{6}{l}{\textbf{libspdm / version negotiation}} \\
\quad Agent-Raw & \excellentcell{}100\% & \goodcell{}50\% & \goodcell{}50\% & \excellentcell{}100\% & \goodcell{}75\% & \quad Agent-Raw & \excellentcell{}100\% & \excellentcell{}100\% & \excellentcell{}100\% & \excellentcell{}100\% & \excellentcell{}100\% \\
\quad Agent-\tla{} & \excellentcell{}100\% & \excellentcell{}100\% & \excellentcell{}100\% & \excellentcell{}100\% & \excellentcell{}100\% & \quad Agent-\tla{} & \excellentcell{}100\% & \excellentcell{}100\% & \goodcell{}50\% & \excellentcell{}100\% & \excellentcell{}83\% \\
\quad Opus & \excellentcell{}100\% & \excellentcell{}100\% & \excellentcell{}100\% & \excellentcell{}100\% & \excellentcell{}100\% & \quad Opus & \excellentcell{}100\% & \excellentcell{}100\% & \excellentcell{}100\% & \excellentcell{}100\% & \excellentcell{}100\% \\
\quad Sonnet & \excellentcell{}100\% & \excellentcell{}100\% & \excellentcell{}100\% & \excellentcell{}100\% & \excellentcell{}100\% & \quad Sonnet & \excellentcell{}100\% & \excellentcell{}100\% & \goodcell{}67\% & \excellentcell{}100\% & \excellentcell{}88\% \\
\quad Haiku & \excellentcell{}100\% & \faircell{}33\% & \faircell{}33\% & 0\% & \faircell{}32\% & \quad Haiku & \excellentcell{}100\% & \faircell{}17\% & \excellentcell{}83\% & 0\% & \faircell{}47\% \\
\addlinespace[2pt]
\multicolumn{6}{l}{\textbf{libspdm / chunking}} & \multicolumn{6}{l}{\textbf{MongoDB / chunk migration}} \\
\quad Agent-Raw & \excellentcell{}100\% & \excellentcell{}83\% & \excellentcell{}83\% & \goodcell{}67\% & \excellentcell{}80\% & \quad Agent-Raw & \excellentcell{}100\% & \goodcell{}71\% & \goodcell{}71\% & \goodcell{}71\% & \goodcell{}76\% \\
\quad Agent-\tla{} & \excellentcell{}100\% & \excellentcell{}83\% & \excellentcell{}83\% & \goodcell{}63\% & \goodcell{}79\% & \quad Agent-\tla{} & \excellentcell{}100\% & \excellentcell{}86\% & \excellentcell{}86\% & \goodcell{}71\% & \excellentcell{}83\% \\
\quad Opus & \excellentcell{}100\% & \excellentcell{}100\% & \excellentcell{}100\% & \excellentcell{}100\% & \excellentcell{}100\% & \quad Opus & \excellentcell{}100\% & \excellentcell{}100\% & \excellentcell{}100\% & \excellentcell{}100\% & \excellentcell{}100\% \\
\quad Sonnet & \excellentcell{}100\% & \excellentcell{}100\% & \goodcell{}50\% & \excellentcell{}86\% & \goodcell{}78\% & \quad Sonnet & \excellentcell{}100\% & \excellentcell{}100\% & \excellentcell{}86\% & \excellentcell{}100\% & \excellentcell{}95\% \\
\quad Haiku & \excellentcell{}100\% & 0\% & \faircell{}17\% & 0\% & \faircell{}21\% & \quad Haiku & \excellentcell{}100\% & \excellentcell{}86\% & \excellentcell{}86\% & 0\% & \goodcell{}58\% \\
\addlinespace[2pt]
\multicolumn{6}{l}{\textbf{libspdm / events}} & \multicolumn{6}{l}{\textbf{MongoDB / Raft reconfig}} \\
\quad Agent-Raw & \excellentcell{}100\% & \goodcell{}67\% & \goodcell{}67\% & \excellentcell{}83\% & \goodcell{}78\% & \quad Agent-Raw & \excellentcell{}100\% & \excellentcell{}83\% & \excellentcell{}83\% & \goodcell{}50\% & \goodcell{}74\% \\
\quad Agent-\tla{} & \excellentcell{}100\% & \goodcell{}67\% & \goodcell{}67\% & \excellentcell{}83\% & \goodcell{}78\% & \quad Agent-\tla{} & \excellentcell{}100\% & \goodcell{}67\% & \goodcell{}67\% & \faircell{}40\% & \goodcell{}62\% \\
\quad Opus & \excellentcell{}100\% & \excellentcell{}100\% & \excellentcell{}100\% & \excellentcell{}100\% & \excellentcell{}100\% & \quad Opus & \excellentcell{}100\% & \excellentcell{}100\% & \excellentcell{}100\% & \excellentcell{}100\% & \excellentcell{}100\% \\
\quad Sonnet & \excellentcell{}100\% & \excellentcell{}100\% & \excellentcell{}100\% & \excellentcell{}100\% & \excellentcell{}100\% & \quad Sonnet & \excellentcell{}100\% & \excellentcell{}100\% & \excellentcell{}100\% & \goodcell{}63\% & \excellentcell{}87\% \\
\quad Haiku & \excellentcell{}100\% & \excellentcell{}100\% & \excellentcell{}83\% & \faircell{}40\% & \goodcell{}73\% & \quad Haiku & \excellentcell{}100\% & \faircell{}33\% & \faircell{}17\% & 0\% & \faircell{}26\% \\
\addlinespace[2pt]
\multicolumn{6}{l}{\textbf{libspdm / key exchange}} & \multicolumn{6}{l}{\textbf{MongoDB / range deletion}} \\
\quad Agent-Raw & \excellentcell{}100\% & \faircell{}43\% & \faircell{}29\% & \faircell{}33\% & \faircell{}43\% & \quad Agent-Raw & \excellentcell{}100\% & \excellentcell{}100\% & \excellentcell{}100\% & \excellentcell{}100\% & \excellentcell{}100\% \\
\quad Agent-\tla{} & \excellentcell{}100\% & \excellentcell{}86\% & \excellentcell{}86\% & \faircell{}33\% & \goodcell{}70\% & \quad Agent-\tla{} & \excellentcell{}100\% & \excellentcell{}100\% & \excellentcell{}100\% & \excellentcell{}100\% & \excellentcell{}100\% \\
\quad Opus & \excellentcell{}100\% & \excellentcell{}100\% & \excellentcell{}100\% & \excellentcell{}100\% & \excellentcell{}100\% & \quad Opus & \excellentcell{}100\% & \excellentcell{}100\% & \excellentcell{}100\% & \excellentcell{}100\% & \excellentcell{}100\% \\
\quad Sonnet & \excellentcell{}100\% & \excellentcell{}100\% & \excellentcell{}100\% & \excellentcell{}100\% & \excellentcell{}100\% & \quad Sonnet & \excellentcell{}100\% & \excellentcell{}100\% & \excellentcell{}100\% & \excellentcell{}100\% & \excellentcell{}100\% \\
\quad Haiku & \excellentcell{}100\% & \faircell{}43\% & \faircell{}43\% & 0\% & \faircell{}36\% & \quad Haiku & 0\% & 0\% & \goodcell{}50\% & 0\% & \faircell{}18\% \\
\addlinespace[2pt]
\multicolumn{6}{l}{\textbf{libspdm / measurement log}} & \multicolumn{6}{l}{\textbf{MongoDB / range preservation}} \\
\quad Agent-Raw & \excellentcell{}100\% & \excellentcell{}83\% & \goodcell{}50\% & \faircell{}43\% & \goodcell{}60\% & \quad Agent-Raw & \excellentcell{}100\% & \goodcell{}57\% & \goodcell{}57\% & \excellentcell{}100\% & \goodcell{}79\% \\
\quad Agent-\tla{} & \excellentcell{}100\% & \excellentcell{}83\% & \goodcell{}67\% & \faircell{}43\% & \goodcell{}66\% & \quad Agent-\tla{} & \excellentcell{}100\% & \faircell{}43\% & \faircell{}14\% & \excellentcell{}100\% & \goodcell{}61\% \\
\quad Opus & \excellentcell{}100\% & \excellentcell{}100\% & \excellentcell{}100\% & \excellentcell{}100\% & \excellentcell{}100\% & \quad Opus & \excellentcell{}100\% & \excellentcell{}100\% & \excellentcell{}100\% & \excellentcell{}100\% & \excellentcell{}100\% \\
\quad Sonnet & \excellentcell{}100\% & \excellentcell{}100\% & \excellentcell{}80\% & \excellentcell{}100\% & \excellentcell{}93\% & \quad Sonnet & \excellentcell{}100\% & \excellentcell{}100\% & \excellentcell{}100\% & \excellentcell{}100\% & \excellentcell{}100\% \\
\quad Haiku & \excellentcell{}100\% & \goodcell{}67\% & \faircell{}33\% & \goodcell{}50\% & \goodcell{}54\% & \quad Haiku & \excellentcell{}100\% & \excellentcell{}100\% & \excellentcell{}86\% & 0\% & \goodcell{}60\% \\
\addlinespace[2pt]
\multicolumn{6}{l}{\textbf{libspdm / measurements}} & \multicolumn{6}{l}{\textbf{MongoDB / sessions}} \\
\quad Agent-Raw & \excellentcell{}100\% & \excellentcell{}100\% & \excellentcell{}100\% & \excellentcell{}83\% & \excellentcell{}94\% & \quad Agent-Raw & \excellentcell{}100\% & \excellentcell{}83\% & \excellentcell{}83\% & \excellentcell{}83\% & \excellentcell{}86\% \\
\quad Agent-\tla{} & \excellentcell{}100\% & \excellentcell{}86\% & \excellentcell{}86\% & \excellentcell{}100\% & \excellentcell{}93\% & \quad Agent-\tla{} & \excellentcell{}100\% & \goodcell{}67\% & \goodcell{}67\% & \excellentcell{}83\% & \goodcell{}78\% \\
\quad Opus & \excellentcell{}100\% & \excellentcell{}100\% & \excellentcell{}100\% & \excellentcell{}100\% & \excellentcell{}100\% & \quad Opus & \excellentcell{}100\% & \excellentcell{}100\% & \excellentcell{}100\% & \excellentcell{}100\% & \excellentcell{}100\% \\
\quad Sonnet & \excellentcell{}100\% & \excellentcell{}100\% & \excellentcell{}100\% & \goodcell{}67\% & \excellentcell{}88\% & \quad Sonnet & \excellentcell{}100\% & \excellentcell{}100\% & \excellentcell{}100\% & \excellentcell{}100\% & \excellentcell{}100\% \\
\quad Haiku & \excellentcell{}100\% & \goodcell{}71\% & \goodcell{}71\% & 0\% & \goodcell{}51\% & \quad Haiku & \excellentcell{}100\% & \excellentcell{}100\% & \excellentcell{}83\% & \goodcell{}75\% & \excellentcell{}85\% \\
\addlinespace[2pt]
\multicolumn{6}{l}{\textbf{libspdm / mutual auth}} & \multicolumn{6}{l}{\textbf{sofa-jraft}} \\
\quad Agent-Raw & \excellentcell{}100\% & \excellentcell{}80\% & \faircell{}20\% & \excellentcell{}100\% & \goodcell{}69\% & \quad Agent-Raw & \excellentcell{}100\% & \excellentcell{}86\% & \goodcell{}71\% & \excellentcell{}100\% & \excellentcell{}88\% \\
\quad Agent-\tla{} & \excellentcell{}100\% & \excellentcell{}100\% & \excellentcell{}100\% & \excellentcell{}100\% & \excellentcell{}100\% & \quad Agent-\tla{} & \excellentcell{}100\% & \excellentcell{}86\% & \goodcell{}57\% & \excellentcell{}100\% & \excellentcell{}83\% \\
\quad Opus & \excellentcell{}100\% & \excellentcell{}100\% & \excellentcell{}100\% & \excellentcell{}100\% & \excellentcell{}100\% & \quad Opus & \excellentcell{}100\% & \excellentcell{}100\% & \excellentcell{}100\% & \excellentcell{}100\% & \excellentcell{}100\% \\
\quad Sonnet & \excellentcell{}100\% & \excellentcell{}100\% & \goodcell{}50\% & \excellentcell{}100\% & \excellentcell{}83\% & \quad Sonnet & \excellentcell{}100\% & \excellentcell{}100\% & \excellentcell{}100\% & \goodcell{}63\% & \excellentcell{}87\% \\
\quad Haiku & \excellentcell{}100\% & \faircell{}20\% & \faircell{}20\% & \excellentcell{}100\% & \goodcell{}60\% & \quad Haiku & \excellentcell{}100\% & \faircell{}43\% & \faircell{}29\% & 0\% & \faircell{}31\% \\
\addlinespace[2pt]
\multicolumn{6}{l}{\textbf{libspdm / PSK exchange}} & \multicolumn{6}{l}{\textbf{Mean}} \\
\quad Agent-Raw & \excellentcell{}100\% & \goodcell{}71\% & \faircell{}43\% & \excellentcell{}88\% & \goodcell{}71\% & \quad Agent-Raw & \excellentcell{}100\% & \goodcell{}79\% & \goodcell{}70\% & \excellentcell{}84\% & \excellentcell{}81\% \\
\quad Agent-\tla{} & \excellentcell{}100\% & \excellentcell{}86\% & \excellentcell{}86\% & \excellentcell{}86\% & \excellentcell{}88\% & \quad Agent-\tla{} & \excellentcell{}100\% & \excellentcell{}82\% & \goodcell{}75\% & \excellentcell{}82\% & \excellentcell{}82\% \\
\quad Opus & \excellentcell{}100\% & \excellentcell{}100\% & \excellentcell{}100\% & \excellentcell{}100\% & \excellentcell{}100\% & \quad Opus & \excellentcell{}100\% & \excellentcell{}100\% & \excellentcell{}100\% & \excellentcell{}100\% & \excellentcell{}100\% \\
\quad Sonnet & \excellentcell{}100\% & \excellentcell{}100\% & \excellentcell{}100\% & \excellentcell{}100\% & \excellentcell{}100\% & \quad Sonnet & \excellentcell{}100\% & \excellentcell{}100\% & \excellentcell{}90\% & \excellentcell{}90\% & \excellentcell{}93\% \\
\quad Haiku & \excellentcell{}100\% & \goodcell{}71\% & \goodcell{}71\% & 0\% & \goodcell{}51\% & \quad Haiku & \excellentcell{}95\% & \goodcell{}56\% & \goodcell{}51\% & \faircell{}17\% & \faircell{}47\% \\
\bottomrule
\end{tabular}
\end{table*}

\begin{table*}[t]
\centering
\footnotesize
\caption{\toreview{\specula-Opus per-module cost (USD) and runtime (minutes) by pipeline phase: P1 (\S\ref{sec:inv}), P2 (\S\ref{sec:specgen}), P3 (\S\ref{sec:conformance}), and P4 (\S\ref{sec:findbugs}); \textbf{Tot} is the per-run total.}}
\label{tab:app-phase-opus}
\resizebox{\textwidth}{!}{%
\setlength{\tabcolsep}{5pt}
\begin{tabular}{ll rrrrr rrrrr}
\toprule
& & \multicolumn{5}{c}{cost (USD)} & \multicolumn{5}{c}{time (min)} \\
\cmidrule(lr){3-7}\cmidrule(lr){8-12}
\textbf{System} & \textbf{Module} & P1 & P2 & P3 & P4 & \textbf{Tot} & P1 & P2 & P3 & P4 & \textbf{Tot} \\
\midrule
Autobahn & BFT consensus & 6.11 & 8.43 & 4.79 & 9.63 & 28.96 & 17 & 38 & 32 & 23 & 110 \\
\midrule
CometBFT & PBTS & 18.66 & 35.72 & 98.17 & 15.28 & 167.83 & 27 & 115 & 232 & 28 & 402 \\
\midrule
\multirow{11}{*}{libspdm} & cert auth & 12.19 & 25.82 & 14.13 & 7.92 & 60.06 & 23 & 121 & 247 & 29 & 420 \\
 & chunking & 6.65 & 13.20 & 3.19 & 6.17 & 29.21 & 14 & 47 & 17 & 17 & 95 \\
 & events & 9.18 & 12.44 & 4.90 & 4.01 & 30.53 & 29 & 43 & 18 & 12 & 102 \\
 & key exchange & 10.15 & 29.92 & 4.93 & 7.30 & 52.30 & 13 & 107 & 48 & 21 & 189 \\
 & measurement log & 5.74 & 23.63 & 8.96 & 5.72 & 44.05 & 18 & 44 & 39 & 12 & 113 \\
 & measurements & 9.06 & 18.38 & 3.67 & 9.68 & 40.79 & 16 & 53 & 15 & 30 & 114 \\
 & mutual auth & 7.61 & 5.81 & 5.31 & 4.33 & 23.06 & 18 & 24 & 11 & 16 & 69 \\
 & PSK exchange & 8.82 & 21.06 & 4.19 & 3.60 & 37.67 & 19 & 59 & 16 & 13 & 107 \\
 & secured messages & 7.23 & 19.44 & 3.43 & 3.56 & 33.66 & 15 & 85 & 12 & 16 & 128 \\
 & session lifecycle & 3.53 & 19.27 & 8.05 & 5.72 & 36.57 & 13 & 87 & 45 & 15 & 160 \\
 & version negotiation & 8.09 & 30.55 & 8.45 & 13.22 & 60.31 & 16 & 116 & 16 & 17 & 165 \\
\midrule
\multirow{5}{*}{MongoDB} & chunk migration & 19.48 & 14.34 & 3.84 & 7.80 & 45.46 & 38 & 56 & 11 & 43 & 148 \\
 & Raft reconfig & 10.75 & 41.92 & 12.01 & 11.04 & 75.72 & 27 & 105 & 37 & 41 & 210 \\
 & range deletion & 9.52 & 14.90 & 3.97 & 5.03 & 33.42 & 19 & 64 & 14 & 31 & 128 \\
 & range preservation & 19.80 & 13.19 & 3.09 & 6.16 & 42.24 & 30 & 94 & 12 & 30 & 166 \\
 & sessions & 15.72 & 16.97 & 4.70 & 3.49 & 40.88 & 29 & 71 & 18 & 16 & 134 \\
\midrule
sofa-jraft & Raft & 13.32 & 47.55 & 11.19 & 9.00 & 81.06 & 17 & 111 & 37 & 34 & 199 \\
\midrule
\multicolumn{2}{l}{\textbf{Mean}} & 10.61 & 21.71 & 11.10 & 7.30 & \textbf{50.73} & 21 & 76 & 46 & 23 & \textbf{166} \\
\bottomrule
\end{tabular}}
\end{table*}

\begin{table*}[t]
\centering
\footnotesize
\caption{\toreview{\specula-Sonnet per-module cost (USD) and runtime (minutes) by pipeline phase (phases as in Table~\ref{tab:app-phase-opus}). Runtimes are active compute time (see Table~\ref{tab:app-time}).}}
\label{tab:app-phase-sonnet}
\resizebox{\textwidth}{!}{%
\setlength{\tabcolsep}{5pt}
\begin{tabular}{ll rrrrr rrrrr}
\toprule
& & \multicolumn{5}{c}{cost (USD)} & \multicolumn{5}{c}{time (min)} \\
\cmidrule(lr){3-7}\cmidrule(lr){8-12}
\textbf{System} & \textbf{Module} & P1 & P2 & P3 & P4 & \textbf{Tot} & P1 & P2 & P3 & P4 & \textbf{Tot} \\
\midrule
Autobahn & BFT consensus & 4.10 & 16.98 & 10.78 & 4.50 & 36.37 & 11 & 74 & 76 & 32 & 193 \\
\midrule
CometBFT & PBTS & 6.37 & 6.05 & 17.40 & 2.96 & 32.78 & 20 & 38 & 148 & 18 & 224 \\
\midrule
\multirow{11}{*}{libspdm} & cert auth & 4.09 & 20.27 & 5.37 & 0.86 & 30.59 & 13 & 102 & 30 & 5 & 150 \\
 & chunking & 4.90 & 7.50 & 12.29 & 7.19 & 31.88 & 21 & 40 & 129 & 36 & 226 \\
 & events & 1.69 & 17.65 & 3.64 & 3.53 & 26.50 & 10 & 86 & 19 & 13 & 128 \\
 & key exchange & 5.07 & 17.09 & 4.12 & 5.29 & 31.58 & 12 & 84 & 27 & 39 & 162 \\
 & measurement log & 6.65 & 18.89 & 4.54 & 5.64 & 35.72 & 23 & 104 & 36 & 30 & 194 \\
 & measurements & 5.58 & 17.24 & 17.97 & 3.25 & 44.05 & 20 & 81 & 166 & 21 & 288 \\
 & mutual auth & 2.61 & 23.47 & 2.71 & 4.55 & 33.34 & 18 & 119 & 20 & 22 & 179 \\
 & PSK exchange & 2.74 & 21.35 & 3.99 & 4.88 & 32.96 & 15 & 116 & 32 & 26 & 189 \\
 & secured messages & 4.72 & 14.19 & 26.21 & 2.42 & 47.54 & 15 & 70 & 133 & 13 & 231 \\
 & session lifecycle & 2.50 & 9.59 & 6.28 & 3.29 & 21.66 & 17 & 63 & 53 & 19 & 152 \\
 & version negotiation & 5.25 & 12.91 & 6.60 & 3.58 & 28.34 & 14 & 73 & 114 & 20 & 222 \\
\midrule
\multirow{5}{*}{MongoDB} & chunk migration & 4.99 & 14.52 & 4.32 & 1.35 & 25.18 & 12 & 117 & 30 & 8 & 166 \\
 & Raft reconfig & 7.80 & 22.17 & 11.00 & 2.32 & 43.30 & 15 & 125 & 93 & 17 & 249 \\
 & range deletion & 9.69 & 4.37 & 6.89 & 1.48 & 22.42 & 14 & 42 & 52 & 11 & 119 \\
 & range preservation & 2.20 & 5.38 & 7.20 & 0.48 & 15.25 & 10 & 42 & 47 & 3 & 103 \\
 & sessions & 5.80 & 6.23 & 9.21 & 2.04 & 23.28 & 17 & 44 & 132 & 15 & 209 \\
\midrule
sofa-jraft & Raft & 7.01 & 7.66 & 13.40 & 0.99 & 29.06 & 16 & 41 & 117 & 6 & 180 \\
\midrule
\multicolumn{2}{l}{\textbf{Mean}} & 4.94 & 13.87 & 9.15 & 3.19 & \textbf{31.15} & 15 & 77 & 77 & 19 & \textbf{188} \\
\bottomrule
\end{tabular}}
\end{table*}

\begin{table*}[t]
\centering
\footnotesize
\caption{\toreview{\specula-Haiku per-module cost (USD) and runtime (minutes) by pipeline phase (phases as in Table~\ref{tab:app-phase-opus}). Runtimes are active compute time (see Table~\ref{tab:app-time}).}}
\label{tab:app-phase-haiku}
\resizebox{\textwidth}{!}{%
\setlength{\tabcolsep}{5pt}
\begin{tabular}{ll rrrrr rrrrr}
\toprule
& & \multicolumn{5}{c}{cost (USD)} & \multicolumn{5}{c}{time (min)} \\
\cmidrule(lr){3-7}\cmidrule(lr){8-12}
\textbf{System} & \textbf{Module} & P1 & P2 & P3 & P4 & \textbf{Tot} & P1 & P2 & P3 & P4 & \textbf{Tot} \\
\midrule
Autobahn & BFT consensus & 0.23 & 0.64 & 1.63 & 0.03 & 2.53 & 2 & 7 & 13 & 0 & 23 \\
\midrule
CometBFT & PBTS & 0.29 & 0.86 & 1.20 & 0.03 & 2.38 & 3 & 10 & 16 & 0 & 28 \\
\midrule
\multirow{11}{*}{libspdm} & cert auth & 0.37 & 1.03 & 1.65 & 0.04 & 3.09 & 4 & 10 & 23 & 1 & 38 \\
 & chunking & 0.23 & 0.75 & 1.53 & 0.03 & 2.54 & 3 & 8 & 13 & 0 & 24 \\
 & events & 0.28 & 0.72 & 1.67 & 0.06 & 2.73 & 3 & 8 & 16 & 1 & 28 \\
 & key exchange & 0.35 & 0.72 & 1.78 & 0.04 & 2.89 & 3 & 8 & 13 & 0 & 24 \\
 & measurement log & 0.26 & 0.86 & 1.67 & 0.27 & 3.06 & 3 & 8 & 15 & 3 & 29 \\
 & measurements & 0.24 & 0.82 & 1.56 & 0.03 & 2.65 & 2 & 9 & 20 & 0 & 32 \\
 & mutual auth & 0.21 & 0.82 & 1.46 & 0.04 & 2.53 & 2 & 8 & 16 & 0 & 26 \\
 & PSK exchange & 0.36 & 1.11 & 1.65 & 0.03 & 3.15 & 4 & 12 & 14 & 0 & 31 \\
 & secured messages & 0.27 & 1.10 & 2.25 & 0.04 & 3.67 & 3 & 10 & 20 & 0 & 33 \\
 & session lifecycle & 0.23 & 0.67 & 2.02 & 0.09 & 3.00 & 2 & 7 & 21 & 1 & 31 \\
 & version negotiation & 0.33 & 0.89 & 2.08 & 0.06 & 3.35 & 3 & 9 & 13 & 1 & 27 \\
\midrule
\multirow{5}{*}{MongoDB} & chunk migration & 0.32 & 0.85 & 0.04 & 0.19 & 1.39 & 3 & 9 & 3 & 2 & 18 \\
 & Raft reconfig & 0.40 & 0.86 & 1.99 & 0.28 & 3.52 & 4 & 10 & 17 & 2 & 33 \\
 & range deletion & 0.27 & 0.97 & 0.99 & 0.35 & 2.57 & 3 & 9 & 12 & 4 & 28 \\
 & range preservation & 0.22 & 0.67 & 1.32 & 0.08 & 2.30 & 2 & 8 & 15 & 1 & 26 \\
 & sessions & 1.47 & 0.78 & 2.54 & 0.98 & 5.78 & 13 & 9 & 18 & 12 & 52 \\
\midrule
sofa-jraft & Raft & 0.70 & 0.43 & 2.16 & 0.04 & 3.33 & 7 & 9 & 21 & 0 & 38 \\
\midrule
\multicolumn{2}{l}{\textbf{Mean}} & 0.37 & 0.82 & 1.64 & 0.14 & \textbf{2.97} & 4 & 9 & 16 & 2 & \textbf{30} \\
\bottomrule
\end{tabular}}
\end{table*}
