# Supplementary material for: Specula: Scaling formal specifications for autonomous model checking of system code
Source: arXiv:2607.25333 source file (2026-08-03)
Supplement: Supplementary file 8 [file 13_evaluated_systems.tex]

\section{Evaluated Systems}
\label{app:systems}

\toreview{%
Table~\ref{tab:systems} lists the \numcases{} systems we evaluated \specula{} on,
    grouped by the system categories of Table~\ref{tab:eval-bugs}, with each
    system's implementation language and source repository.%
}

\begin{table*}[t]
\centering
\footnotesize
\setlength{\tabcolsep}{4pt}
\caption{\toreview{The \numcases{} evaluated systems, grouped by system category
  (as in Table~\ref{tab:eval-bugs}), with implementation language and source
  repository.}}
\label{tab:systems}
\begin{tabular}[t]{l l l}
\toprule
\textbf{System} & \textbf{Language} & \textbf{Repository} \\
\midrule
\multicolumn{3}{l}{\textbf{Consensus Systems (31)}} \\
\midrule
Aptos             & Rust   & \href{https://github.com/aptos-labs/aptos-core}{\texttt{aptos-labs/aptos-core}} \\
async-raft        & Rust   & \href{https://github.com/async-raft/async-raft}{\texttt{async-raft/async-raft}} \\
Autobahn          & Rust   & \href{https://github.com/neilgiri/autobahn-artifact}{\texttt{neilgiri/autobahn-artifact}} \\
Babylon           & Go     & \href{https://github.com/babylonlabs-io/babylon}{\texttt{babylonlabs-io/babylon}} \\
Besu QBFT         & Java   & \href{https://github.com/hyperledger/besu}{\texttt{hyperledger/besu}} \\
braft             & C++    & \href{https://github.com/baidu/braft}{\texttt{baidu/braft}} \\
CometBFT          & Go     & \href{https://github.com/cometbft/cometbft}{\texttt{cometbft/cometbft}} \\
dotNext           & C\#    & \href{https://github.com/dotnet/dotNext}{\texttt{dotnet/dotNext}} \\
Dragonboat        & Go     & \href{https://github.com/lni/dragonboat}{\texttt{lni/dragonboat}} \\
eliben-raft       & Go     & \href{https://github.com/eliben/raft}{\texttt{eliben/raft}} \\
Epaxos            & Go     & \href{https://github.com/imdea-software/swiftpaxos}{\texttt{imdea-software/swiftpaxos}} \\
etcd raft         & Go     & \href{https://github.com/etcd-io/raft}{\texttt{etcd-io/raft}} \\
go-algorand       & Go     & \href{https://github.com/algorand/go-algorand}{\texttt{algorand/go-algorand}} \\
goraft            & Go     & \href{https://github.com/goraft/raft}{\texttt{goraft/raft}} \\
hashicorp/raft    & Go     & \href{https://github.com/hashicorp/raft}{\texttt{hashicorp/raft}} \\
HotShot           & Rust   & \href{https://github.com/EspressoSystems/HotShot}{\texttt{EspressoSystems/HotShot}} \\
N2Paxos           & Go     & \href{https://github.com/imdea-software/swiftpaxos}{\texttt{imdea-software/swiftpaxos}} \\
nebula            & C++    & \href{https://github.com/vesoft-inc/nebula}{\texttt{vesoft-inc/nebula}} \\
NuRaft            & C++    & \href{https://github.com/eBay/NuRaft}{\texttt{eBay/NuRaft}} \\
rabbitmq/ra       & Erlang & \href{https://github.com/rabbitmq/ra}{\texttt{rabbitmq/ra}} \\
raft-java         & Java   & \href{https://github.com/wenweihu86/raft-java}{\texttt{wenweihu86/raft-java}} \\
RedisRaft         & C      & \href{https://github.com/RedisLabs/redisraft}{\texttt{RedisLabs/redisraft}} \\
RethinkDB         & C++    & \href{https://github.com/rethinkdb/rethinkdb}{\texttt{rethinkdb/rethinkdb}} \\
ScyllaDB          & C++    & \href{https://github.com/scylladb/scylladb}{\texttt{scylladb/scylladb}} \\
sofa-jraft        & Java   & \href{https://github.com/sofastack/sofa-jraft}{\texttt{sofastack/sofa-jraft}} \\
Solana            & Rust   & \href{https://github.com/anza-xyz/agave}{\texttt{anza-xyz/agave}} \\
\bottomrule
\end{tabular}
\hspace{12pt}
\begin{tabular}[t]{l l l}
\toprule
\textbf{System} & \textbf{Language} & \textbf{Repository} \\
\midrule
\multicolumn{3}{l}{\textbf{Consensus Systems (cont.)}} \\
\midrule
Substrate         & Rust   & \href{https://github.com/paritytech/substrate}{\texttt{paritytech/substrate}} \\
Sui               & Rust   & \href{https://github.com/MystenLabs/sui}{\texttt{MystenLabs/sui}} \\
SwiftPaxos        & Go     & \href{https://github.com/imdea-software/swiftpaxos}{\texttt{imdea-software/swiftpaxos}} \\
tikv/raft-rs      & Rust   & \href{https://github.com/tikv/raft-rs}{\texttt{tikv/raft-rs}} \\
willemt/raft      & C      & \href{https://github.com/willemt/raft}{\texttt{willemt/raft}} \\
\midrule
\multicolumn{3}{l}{\textbf{Concurrent Data Structures (8)}} \\
\midrule
arc-swap          & Rust   & \href{https://github.com/vorner/arc-swap}{\texttt{vorner/arc-swap}} \\
crossbeam         & Rust   & \href{https://github.com/crossbeam-rs/crossbeam}{\texttt{crossbeam-rs/crossbeam}} \\
dpdk-ring         & C      & \href{https://github.com/DPDK/dpdk}{\texttt{DPDK/dpdk}} \\
kanal             & Rust   & \href{https://github.com/fereidani/kanal}{\texttt{fereidani/kanal}} \\
left-right        & Rust   & \href{https://github.com/jonhoo/left-right}{\texttt{jonhoo/left-right}} \\
papaya            & Rust   & \href{https://github.com/ibraheemdev/papaya}{\texttt{ibraheemdev/papaya}} \\
scc               & Rust   & \href{https://github.com/wvwwvwwv/scalable-concurrent-containers}{\texttt{wvwwvwwv/scalable-}} \\
                  &        & \href{https://github.com/wvwwvwwv/scalable-concurrent-containers}{\texttt{concurrent-containers}} \\
tokio-broadcast   & Rust   & \href{https://github.com/tokio-rs/tokio}{\texttt{tokio-rs/tokio}} \\
\midrule
\multicolumn{3}{l}{\textbf{Database Systems (1)}} \\
\midrule
MongoDB           & C++    & \href{https://github.com/mongodb/mongo}{\texttt{mongodb/mongo}} \\
\midrule
\multicolumn{3}{l}{\textbf{Network Systems (4)}} \\
\midrule
sonic-buildimage iccpd & C & \href{https://github.com/sonic-net/sonic-buildimage}{\texttt{sonic-net/sonic-buildimage}} \\
sonic-dash-ha     & Rust   & \href{https://github.com/sonic-net/sonic-dash-ha}{\texttt{sonic-net/sonic-dash-ha}} \\
sonic-linkmgrd    & C++    & \href{https://github.com/sonic-net/sonic-linkmgrd}{\texttt{sonic-net/sonic-linkmgrd}} \\
sonic-swss        & C++    & \href{https://github.com/sonic-net/sonic-swss}{\texttt{sonic-net/sonic-swss}} \\
\midrule
\multicolumn{3}{l}{\textbf{Parallel Runtimes (2)}} \\
\midrule
libgomp (GCC)     & C      & \href{https://github.com/gcc-mirror/gcc}{\texttt{gcc-mirror/gcc}} \\
LLVM libomp       & C++    & \href{https://github.com/llvm/llvm-project}{\texttt{llvm/llvm-project}} \\
\midrule
\multicolumn{3}{l}{\textbf{Security Protocols (2)}} \\
\midrule
libspdm           & C      & \href{https://github.com/DMTF/libspdm}{\texttt{DMTF/libspdm}} \\
spdm-rs           & Rust   & \href{https://github.com/ccc-spdm-tools/spdm-rs}{\texttt{ccc-spdm-tools/spdm-rs}} \\
\bottomrule
\end{tabular}
\end{table*}
