# Supplementary material for: Specula: Scaling formal specifications for autonomous model checking of system code
Source: arXiv:2607.25333 source file (2026-08-03)
Supplement: Supplementary file 9 [file proof.tex]

\section{Analysis of the Validation Loops}
\label{app:convergence}

\subsection{Purpose}
\label{app:conv-purpose}

\toreview{%
The conformance loop (\S\ref{sec:conformance}) and the confirmation loop (\S\ref{sec:findbugs})
    must reach sound outcomes even though every input they consume can be wrong.
Section~\ref{sec:evo-loop} describes what evidence \specula gathers at each step
    and how the loops use it.
Under the assumption of \S\ref{app:conv-assumption}, we prove two claims and discuss a third:%
}

\begin{itemize}[leftmargin=1.4em, itemsep=3pt, topsep=3pt]
  \item \toreview{\textbf{Soundness} (proved). No real bug is silently discarded.
    In the worst case it is deferred to a developer.}
  \item \toreview{\textbf{Correctness} (proved). Wherever the loops settle,
    the model conforms to the implementation and the surviving invariants are correct.}
  \item \toreview{\textbf{Convergence} (discussed). We do not prove that the loops settle.
    We discuss the question and argue, from how \specula is built and from its behavior in practice,
    that they do.}
\end{itemize}

\subsection{Preliminaries}
\label{app:conv-prelim}

\toreview{%
\specula model checks a model $M$ against a set of invariants.
We separate implementation states from the states of $M$,
    and write $\alpha(c)$ for the model state that represents an implementation state $c$.
The map $\alpha$ is many to one: a model state may represent many implementation states.%
}

\toreview{%
Let $\mathcal{R}$ be the set of \emph{reachable} implementation states,
    those the implementation reaches in some execution, possibly under injected faults.
A model state $s$ is \emph{reachable} when $s \in \alpha(\mathcal{R})$,
    that is $s = \alpha(c)$ for some $c \in \mathcal{R}$, and \emph{unreachable} otherwise.%
}

\toreview{%
Legality is fixed by the system's intended semantics, the design's decision about which behaviors
    are permitted, and is defined first on implementation states:
    $\mathrm{legal}(c)$ holds when the intended semantics permit $c$.
It lifts to $M$ along $\alpha$: when the implementation states a model state represents agree on
    legality, $\mathrm{legal}(s)$ takes their common value.
A \emph{real bug} is a reachable illegal state, an $s \in \alpha(\mathcal{R})$ with $\neg\,\mathrm{legal}(s)$.%
}

\toreview{%
A \emph{violation} is a pair $(s, \varphi)$ where $M$ reaches $s$ and $\neg\varphi(s)$.
Exactly one case holds:%
}

\begin{itemize}[leftmargin=1.4em, itemsep=3pt, topsep=3pt]
  \item \toreview{$s \notin \alpha(\mathcal{R})$: the violation is a \emph{model artifact}.}
  \item \toreview{$s \in \alpha(\mathcal{R})$ and $\mathrm{legal}(s)$: the invariant $\varphi$ is \emph{wrong} at $s$.}
  \item \toreview{$s \in \alpha(\mathcal{R})$ and $\neg\,\mathrm{legal}(s)$: $(s,\varphi)$ exposes a \emph{real bug}.}
\end{itemize}

\toreview{%
Adjudicating $(s,\varphi)$ yields one of three outcomes, each asserting the matching case, or a deferral:%
}

\begin{itemize}[leftmargin=1.4em, itemsep=2pt, topsep=3pt]
  \item \toreview{\textbf{Model repair} asserts $s \notin \alpha(\mathcal{R})$ and tightens $M$.}
  \item \toreview{\textbf{Invariant revision} asserts $\mathrm{legal}(s)$ and corrects $\varphi$.}
  \item \toreview{\textbf{Bug report} asserts $s \in \alpha(\mathcal{R}) \wedge \neg\,\mathrm{legal}(s)$ and reports the bug.}
\end{itemize}

\toreview{%
When the evidence supports no assertion, $(s,\varphi)$ is \emph{deferred} to a developer.
Model repair and invariant revision \emph{discharge} $(s,\varphi)$, ruling it not a bug.
The two loops reach these outcomes between them. Their only added case is a bug whose downstream
    consequence is masked, which is still a bug report and needs no separate treatment.%
}

\subsection{The core assumption}
\label{app:conv-assumption}

\toreview{%
We do not assume the agent can find the evidence a case needs, even when it exists
    in the code or its history.
The agent may search and miss it.
We do not assume it reads the evidence it finds correctly.
We do not assume it is ever certain.
In any of these the agent cannot cite supporting evidence, so it commits no judgment,
    and the violation stays a candidate bug.%
}

\toreview{%
We assume one thing, and only under three premises that \specula enforces.%
}

\toreview{%
\para{Premise 1 (evidence is supplied).}
For every violation it adjudicates, \specula places the relevant evidence before the agent:
    the trace under replay, the cited code and development history,
    and the output of the reproduction harness.
Where the evidence to decide a case exists, the agent has access to it.%
}

\toreview{%
\para{Premise 2 (evidence is required).}
Every judgment the agent commits to, whether a model repair, an invariant revision,
    or a bug report, must cite the evidence that supports it: the code, a commit, an issue,
    a comment, a test, or, for a bug report, a reproduction (\S\ref{sec:evo-loop}).
A judgment with no such evidence does not take effect.%
}

\toreview{%
\para{Premise 3 (fallback exists).}
When the agent commits no judgment, for any reason,
    the violation is kept as a candidate bug rather than dropped,
    and if it is never discharged it is deferred to a developer.%
}

\toreview{%
\para{Assumption (no judgment against the evidence).}
Under these premises, the agent commits an outcome only when its evidence does not refute the
    assertion that outcome makes.
It will not fabricate evidence, and it will not cite real evidence for a conclusion that evidence denies.
The assumption forbids asserting against the evidence. It never forces the agent to assert.%
}

\subsection{Soundness}
\label{app:conv-soundness}

\begin{proposition}[Soundness]
\label{prop:soundness}
\toreview{A real bug is never discharged, and so is reported or deferred to a developer.}
\end{proposition}

\begin{proof}
\toreview{%
Let $(s,\varphi)$ be a real bug, so $s \in \alpha(\mathcal{R})$ and $\neg\,\mathrm{legal}(s)$.
It leaves the candidate set only by a discharge, a model repair or an invariant revision,
    and we rule out both.%
}

\toreview{%
\para{Model repair} asserts $s \notin \alpha(\mathcal{R})$, which is false, since $s$ is reachable.
To discharge $(s,\varphi)$ a repair would have to stop $M$ from reaching $s$.
But $s$ is reached by a real execution, which trace validation replays against the tightened $M$.
The tightened $M$ rejects that execution, so the repair fails validation and is undone,
    and $(s,\varphi)$ returns.
A repair that does not stop $M$ from reaching $s$ leaves model checking to flag $(s,\varphi)$ again.
A repair that enlarges $M$ only adds more to check, which bears on convergence,
    not soundness (\S\ref{app:conv-converge}).%
}

\toreview{%
\para{Invariant revision} asserts $\mathrm{legal}(s)$, which is false here.
The assertion rests on the system's own evidence, the code, its history, a comment, a test,
    not on the invariant, so a wrong invariant cannot license its own correction.
Since the evidence shows the system forbids $s$, by the assumption the agent does not assert
    $\mathrm{legal}(s)$, and the bug is not revised away.%
}

\toreview{%
Neither discharge stands, so by Premise~3 the violation is reported or deferred.%
}
\end{proof}

\subsection{Correctness}
\label{app:conv-correctness}

\toreview{%
\para{Opposed directions.}
The conformance loop pulls $M$ two ways.
Trace validation pulls toward admitting more: a rejected real trace makes $M$ widen to include it.
Model checking pulls toward admitting less: a spurious violation makes $M$ narrow to exclude it.
The two targets meet at an $M$ that admits the behavior its traces exercise
    and raises no spurious violation, which we call conformant.%
}

\begin{proposition}[Correctness]
\label{prop:correctness}
\toreview{%
Suppose the loops settle at a conformant $M$ on which no repair or revision fires.
Then no surviving violation is a model artifact, and every invariant still in force is correct,
    except possibly one whose violation was deferred to a developer.%
}
\end{proposition}

\begin{proof}
\toreview{%
A conformant $M$ raises no spurious violation, so no surviving violation has $s \notin \alpha(\mathcal{R})$.
Suppose an invariant $\varphi$ in force is wrong at a reachable state,
    so $s \in \alpha(\mathcal{R})$, $\mathrm{legal}(s)$, and $\neg\varphi(s)$.
Then $(s,\varphi)$ is a live violation whose only discharge is an invariant revision:
    model repair asserts $s \notin \alpha(\mathcal{R})$ and bug report asserts $\neg\,\mathrm{legal}(s)$,
    both false and refused by the assumption.
If the legality evidence is available, that revision fires, against $\varphi$ being in force.
    Otherwise the violation is deferred.
So a wrong invariant in force has a deferred violation.
Finally a correct invariant is never revised, since by the assumption no evidence asserts
    $\mathrm{legal}(s)$ of an illegal $s$.%
}
\end{proof}

\subsection{Convergence}
\label{app:conv-converge}

\toreview{%
We cannot prove the loops always settle.
A repair is not final: even after it passes trace validation it may introduce an illegal state,
    which is why model checking runs again after each repair,
    and the agent could in principle propose flawed repairs without end.
What works against this is the record \specula keeps of every repair and its outcome.
The record lets the agent see a past mistake and not repeat it,
    and see the consequence each repair had, which guides a better repair.
We do not claim it shrinks the room for error to nothing.
We observe that, with the record in place,
    \specula's loops settled in our evaluation rather than oscillating.
Where the agent cannot make progress, the violation is deferred to a developer,
    so the cost of non-convergence is a deferral, never a lost bug.%
}
