# Supplementary material for: Specula: Scaling formal specifications for autonomous model checking of system code
Source: arXiv:2607.25333 source file (2026-08-03)
Supplement: Supplementary file 10 [file 01_mcps.tex]

\section{\specula MCPs}
\label{app:tools}

Table \ref{tab:tools} describes the custom MCPs provided to \specula.
They remain available to the agent across all phases but are specifically invoked only in certain phases.

\begin{table}[]
\centering
\caption{MCPs provided to \specula}
\label{tab:tools}
\begin{tabular}{lll}
\hline
\textbf{Tool}            & \textbf{Purpose}                                                                        & \textbf{\begin{tabular}[c]{@{}l@{}}Focused\\ Usage\end{tabular}} \\ \hline
\textsf{tla2sany}        & Syntax validation                                                                       & Phase 2                \\ \hline
\textsf{spec\_analyzer}  & \begin{tabular}[c]{@{}l@{}}Static analysis to verify\\ actions are atomic\end{tabular}  & Phase 2                \\ \hline
\textsf{trace\_debugger} & \begin{tabular}[c]{@{}l@{}}Trace validation,\\ step-through debugger tools\end{tabular} & Phase 3                \\ \hline
\textsf{MC\_summary} & \begin{tabular}[c]{@{}l@{}}State comparison, expression\\ eval at intermediate states\end{tabular} & Phase 3 \\ \hline
\end{tabular}
\end{table}
