# Supplementary material for: Specula: Scaling formal specifications for autonomous model checking of system code
Source: arXiv:2607.25333 source file (2026-08-03)
Supplement: Supplementary file 11 [file 04_bug_distribution.tex]

\section{RQ1: Bug Distribution By Language}
\label{app:language-bugs}

Table \ref{tab:language-bugs} describes the number of reported and confirmed bugs per language, as well as the number of repositories in that language tested.
The language with the highest average bugs-per-project ratio was Erlang (7), though this may not be representative as we only ran \specula on one Erlang repository.
The individual project with the highest bug count was CometBFT (21 bugs, Go), followed by MongoDB (19 bugs, C++).
The language with the lowest average bugs-per-project ratio was C++ (3.8), as its many consensus implementations each yielded relatively few bugs.

\begin{table}[]
\centering
\caption{Number of reported and confirmed bugs and number of target repositories tested per language.}
\label{tab:language-bugs}
\begin{tabular}{llll}
\hline
\textbf{Language} & \textbf{Reported} & \textbf{Confirmed} & \textbf{Repos} \\ \hline
Rust   & 87 & 40 & 20 \\ \hline
C++    & 45 & 8  & 12 \\ \hline
Go     & 52 & 8  & 11 \\ \hline
C      & 39 & 18 & 6  \\ \hline
Java   & 18 & 5  & 3  \\ \hline
Erlang & 7  & 7  & 1  \\ \hline
C\#    & 4  & 2  & 1  \\ \hline
\end{tabular}
\end{table}
