# Supplementary material for: Specula: Scaling formal specifications for autonomous model checking of system code
Source: arXiv:2607.25333 source file (2026-08-03)
Supplement: Supplementary file 12 [file 05_invariant_depths.tex]

\section{RQ1: Bug Invariant Violation Depths}
\label{app:depths}

Figure \ref{fig:rq1-depths} depicts the distribution of \tla model checking invariant violation depths for the bugs reported in Section \ref{sec:rq1}.
The median depth was 11 steps, the 5th percentile was 4 steps, and the 95th percentile was 56.60 steps.
Note that some bugs reported did not have an associated invariant violation (e.g., minor typos, deadlock), hence not all \numbugs{} bugs are represented here.

\begin{figure}[]
    \centering
    \includegraphics[width=\linewidth]{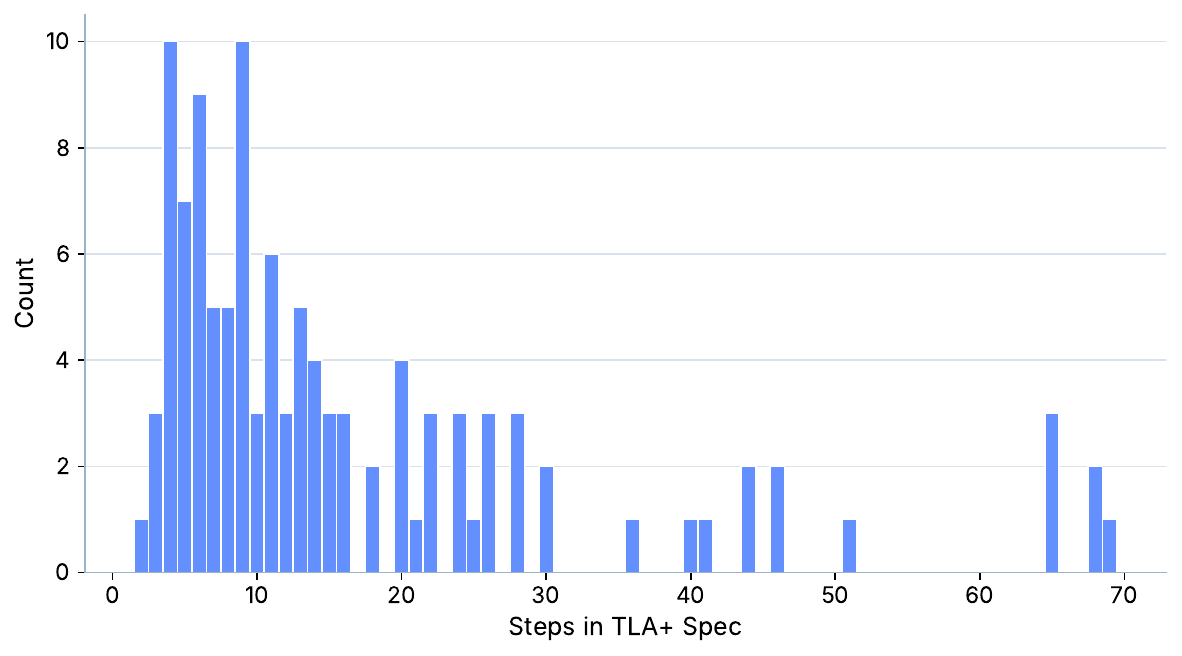}
    \caption{Distribution of the number of \tla model checking steps before invariant violation occurred.}
    \label{fig:rq1-depths}
\end{figure}
