# Supplementary material for: Specula: Scaling formal specifications for autonomous model checking of system code
Source: arXiv:2607.25333 source file (2026-08-03)
Supplement: Supplementary file 13 [file 08_cost_runtime.tex]

\section{RQ4: \specula Cost and Runtime}
\label{app:rq4-cost-runtime}

Figure \ref{fig:rq4-cost-time} illustrates the cost and runtime breakdown per-phase, comparing between the agent baselines and \specula's different configurations. The figure does not include a separate \textsf{no-phase-4} bar since it would be identical to the \textsf{\specula} bar without the final phase.

\begin{figure*}
\setlength\columnsep{10pt}
\begin{multicols}{2}
    \noindent
    \includegraphics[width=\linewidth]{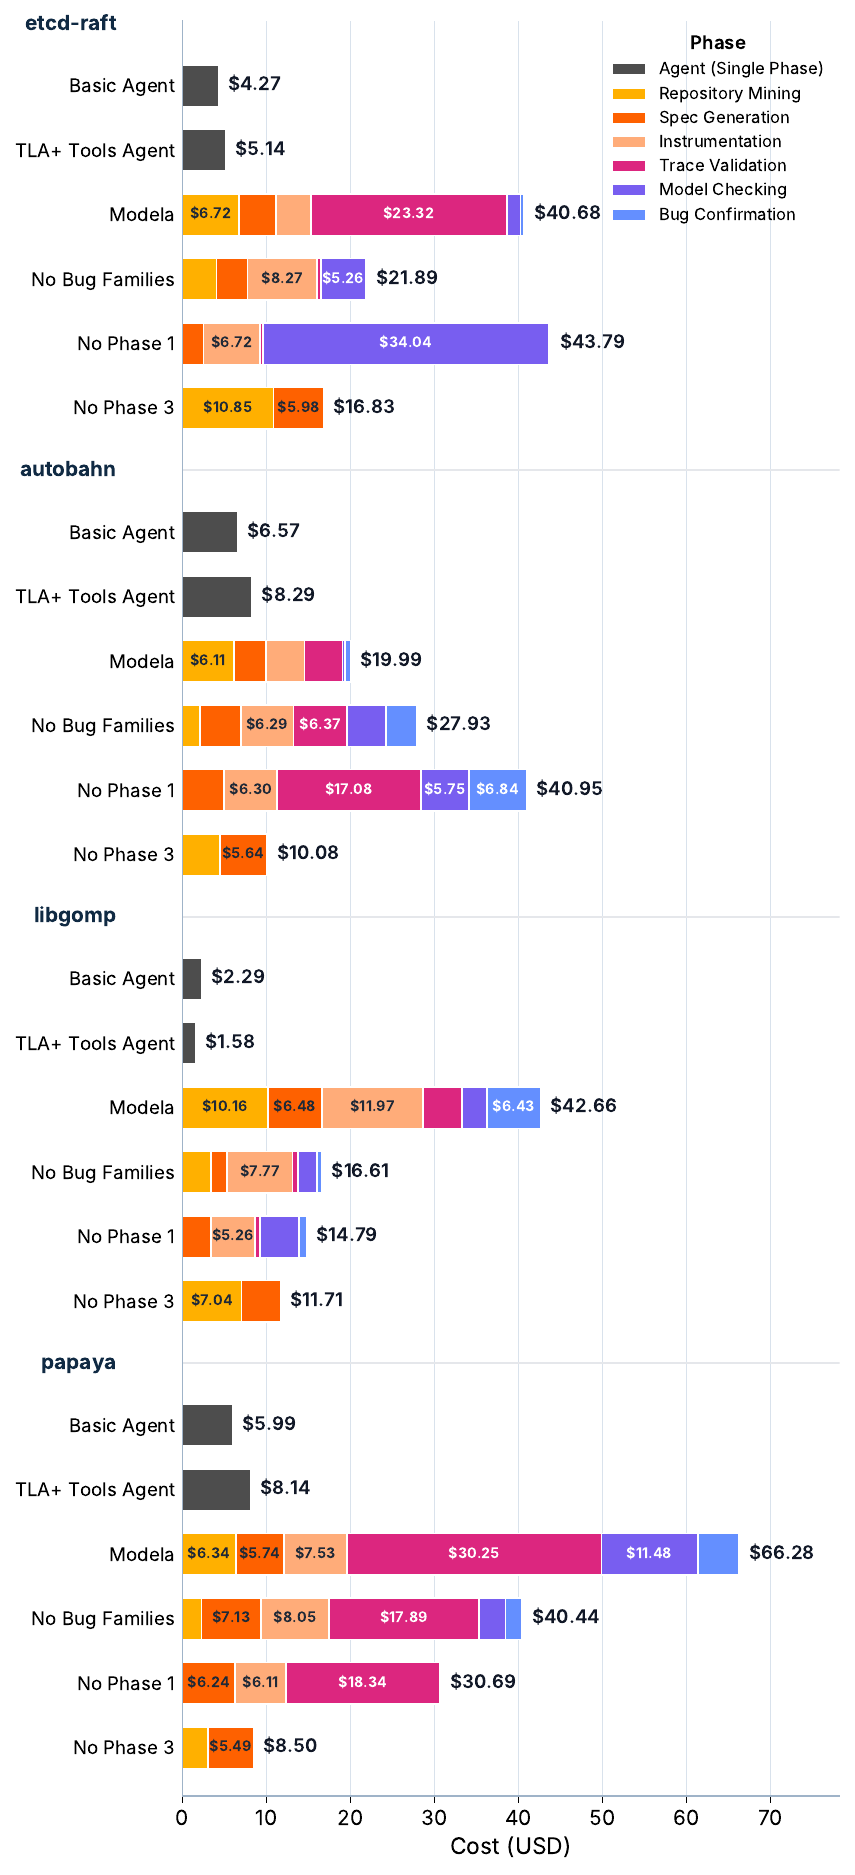}\par
    \includegraphics[width=\linewidth]{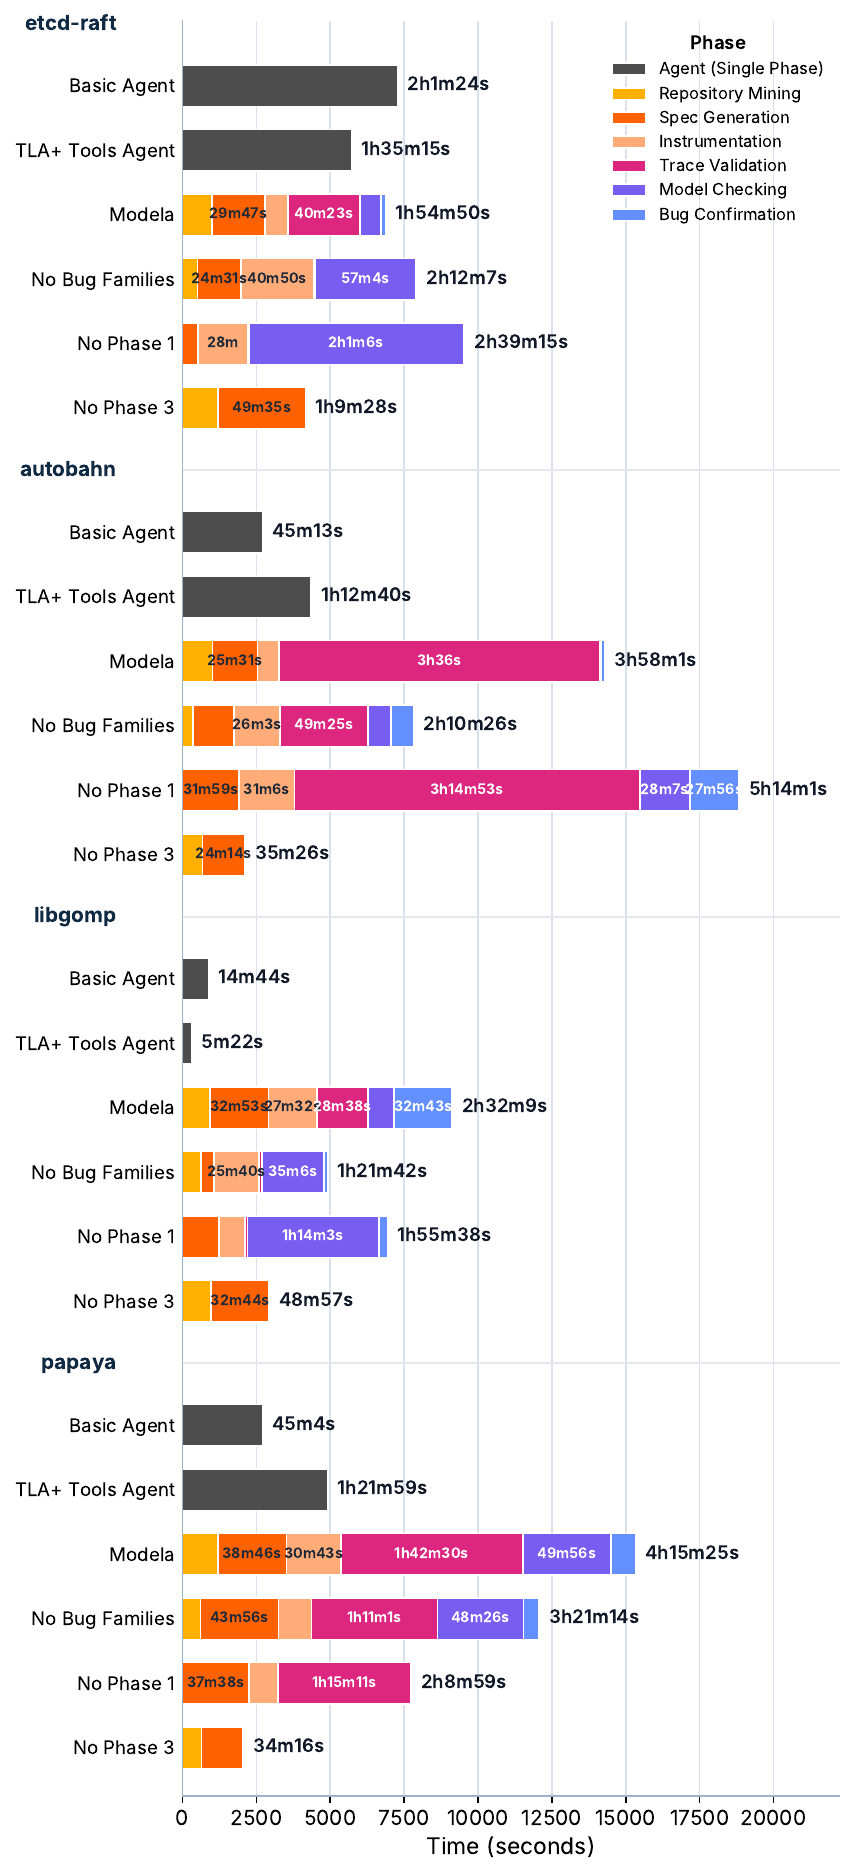}\par
    \end{multicols}
\caption{Cost (in USD) and runtime per phase per agent configuration.}
    \label{fig:rq4-cost-time}
\end{figure*}
