# Supplementary material for: Specula: Scaling formal specifications for autonomous model checking of system code
Source: arXiv:2607.25333 source file (2026-08-03)
Supplement: Supplementary file 14 [file 12_language_bugs.tex]

\section{Bugs by Implementation Language}
\label{app:language-bugs}

\toreview{%
Table~\ref{tab:language-bugs} breaks the \numbugs{} bugs of \S\ref{sec:eval-bugs}
    down by the implementation language of the \numcases{} systems.%
}

\begin{table}[t]
\centering
\small
\caption{\toreview{Bugs \specula{} found by implementation language, sorted by the
  average number of bugs per system (Avg.). New (conf.) and Known as in
  Table~\ref{tab:eval-bugs}.}}
\label{tab:language-bugs}
% Derived from scripts/specula_bug_restat.csv. Systems merged to the 48-system
% corpus convention: HashiCorp Raft x2 -> 1, crossbeam x3 -> 1, Aptos x2 -> 1,
% sonic-swss family x4 -> 1. Totals must agree with Table tab:eval-bugs and
% \numcases / \numnewbugs (\numconfirmed) / \numknownbugs / \numbugs in preamble.tex.
\begin{tabular}{l r r r r r}
\toprule
\textbf{Language} & \textbf{Systems} & \textbf{New (conf.)} & \textbf{Known}
  & \textbf{Total} & \textbf{Avg.} \\
\midrule
C      &  6 &  44 (18) &  2 &  46 & 7.7 \\
Erlang &  1 &   7 (7)  &  0 &   7 & 7.0 \\
Java   &  3 &  14 (4)  &  4 &  18 & 6.0 \\
Rust   & 17 &  67 (28) & 20 &  87 & 5.1 \\
C++    &  9 &  34 (2)  &  7 &  41 & 4.6 \\
Go     & 11 &  37 (7)  &  9 &  46 & 4.2 \\
C\#    &  1 &   4 (2)  &  0 &   4 & 4.0 \\
\midrule
\textbf{Total} & 48 & 207 (68) & 42 & 249 & 5.2 \\
\bottomrule
\end{tabular}
\end{table}
